# Supplementary material for: Quantum coherent spin-electric control in a molecular nanomagnet at clock transitions
Source: arXiv:2005.01029 ancillary file (2021-07-21)
Supplement: Supplementary file 1 [file HoW10_SI_20Jul2021.pdf]

# Supplementary Information:
# Quantum coherent spin-electric control in a molecular nanomagnet at clock transitions

Junjie Liu,[1,*] Jakub Mrozek,[1] Aman Ullah,[2] Yan Duan,[2] José J. Baldoví,[2]
Eugenio Coronado,[2] Alejandro Gaita-Ariño,[2,†] and Arzhang Ardavan[1,‡]

[1]*CAESR, Department of Physics, University of Oxford, The Clarendon Laboratory, Parks Road, Oxford OX1 3PU, UK*
[2]*Instituto de Ciencia Molecular (ICMol), Universitat de València, Paterna, Spain*

## I. EXPERIMENTAL PULSE SEQUENCES

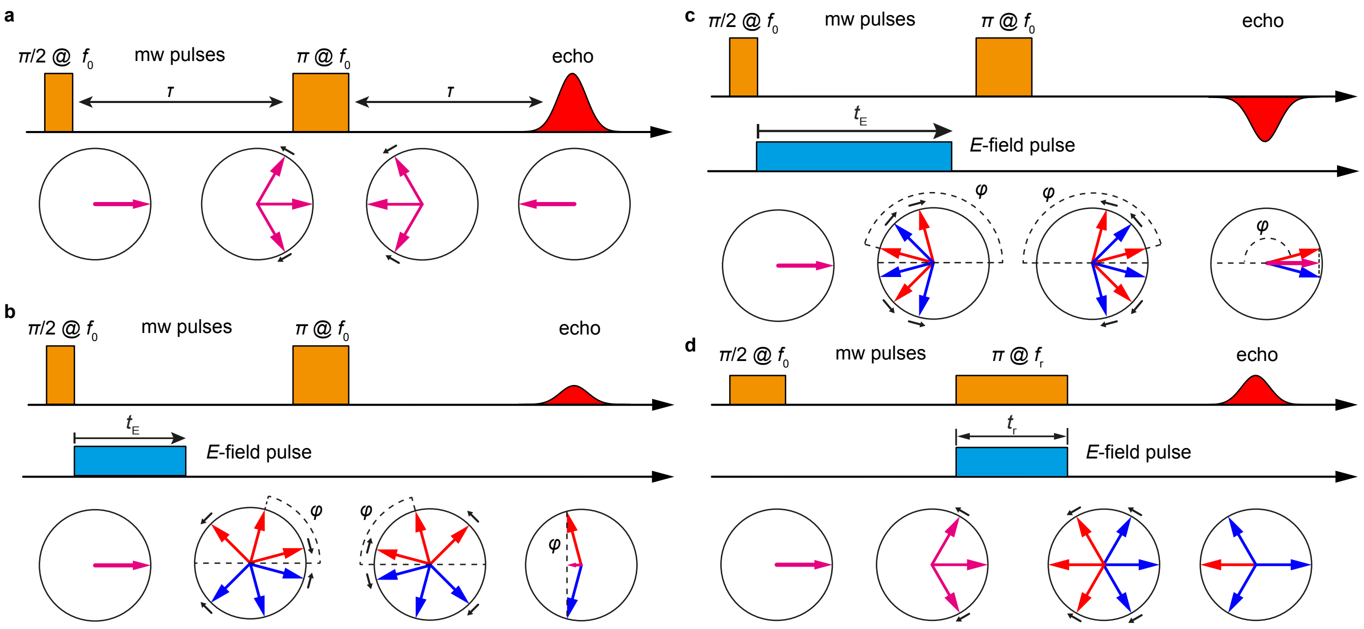


FIG. S1. Pulse sequences, together with the spin evolution schemes (in the $xy$ plane of the Bloch sphere), depicting the formation of the spin echoes. In all sequences, the initial $\pi/2$ pulse rotates the spins parallel to the $x$ axis. The blue and red arrows represent the spins for the crystallographically inequivalent $HoW_{10}$ molecules related by inversion symmetry. The magenta arrows correspond to the summation of the red and blue arrows. **a**, Standard Hahn-echo sequence without any electric field. The evolutions of the blue and red spins are identical in the absence of an $E$-field pulse. The phase accumulation induced by static inhomogeneous (external or internal) magnetic fields in the first free evolution period is inverted by the $\pi$ refocusing pulse. The spin echo is expected to form in the in-phase channel at $t = 2\tau$. **b**, An $E$-field pulse, applied immediately after the initial $\pi/2$ microwave pulse, increases (decreases) the precessing frequency for the red (blue) spins due to a linear spin-electric coupling (SEC) in $HoW_{10}$ molecules. This leads to a $+\psi$ or $-\psi$ phase shift for the red and blue spins respectively, with $\psi = \delta f \times t_{\mathrm{E}}$. The final echo is the summation of both red and blue spins and remains strictly in the in-phase channel, while its intensity ($I$) varies as $I \propto \cos(\delta f t_{\mathrm{E}})$. **c**, Upon further increasing the duration and/or amplitude of the $E$-field pulse, $\psi$ increases, reversing the polarity of the spin echo. **d**, Electric-field-assisted spin selection. An $E$-field pulse is applied simultaneously with the refocusing $\pi$ pulse, lifting the degeneracy in the ESR transitions of the two inversion-related subpopulations. When the frequency difference between the two subpopulations is larger than the excitation bandwidth of the $\pi$ pulse, i.e. $|2\delta f| > 1/t_{\mathrm{r}}$ (where $t_{\mathrm{r}}$ is the duration of the $\pi$ pulse), only one subpopulation of the $HoW_{10}$ spins (red arrows) is refocused by a $\pi$ pulse with the frequency of $f_{\mathrm{r}} = f_0 + \delta f$. The other subpopulation (blue arrows) does not form an echo because the phase accumulated owing to inhomogeneities is not refocused by the $\pi$ pulse and instead accumulates monotonically throughout the pulse sequence. Therefore, the detected echo is comprised of only one subpopulation of the molecules.

* junjie.liu@physics.ox.ac.uk
† Alejandro.Gaita@uv.es
‡ arzhang.ardavan@physics.ox.ac.uk

## II. MOLECULAR STRUCTURE FOR $HoW_{10}$

The $Ho^{3+}$ ion is octa-coordinated by four oxygen atoms from each of the monolacunary Lindqvist moieties $[W_5O_{18}]^{6-}$ in a slightly distorted square antiprismatic geometry, providing an approximate $D_{4d}$ symmetry for the $Ho^{3+}$ centre (see Fig 1a in the main text). The deviation from the $D_{4d}$ symmetry of the first coordination sphere of the $Ho^{3+}$ centre can be described by the dihedral and the axial distortions. The dihedral distortion is the average of the absolute deviation of the skew angles $\theta$ from the ideal value (45° for $D_{4d}$). There are four possible skew angles which can be formed by the four independent pairs of O-Ho-O planes. The axial distortion is defined as the off-centre vertical displacement of the $Ho^{3+}$ centre, expressed as $d = (h - h')/2$, where $h$ and $h'$ are the distances from the $Ho^{3+}$ atom to the mean planes passing through the square bases of the antiprisms. The dihedral and the axial distortions for three different temperatures (100 K, 150 K and 200 K) are listed in Table S1. The single crystal structures of the same sample at three different temperatures (100 K, 150 K and 200 K) were determined and resolved in this work. CSD 2036358-2036360 contains the supplementary crystallographic data for this paper. These data can be obtained free of charge via `http://www.ccdc.cam.ac.uk/structures`, by emailing `data_request@ccdc.cam.ac.uk`, or by contacting The Cambridge Crystallographic Data Centre, 12 Union Road, Cambridge CB2 1EZ, UK; fax: +44 1223 336033.

On the basis of the crystal data and the optimized structure data, the quantification of the distortion is carried out by utilization of continuous shape measurement (CShMs) calculations using the SHAPE 2.1 software [S1, S2]. The values given by the Shape software are equal to 0, corresponding to the perfect polyhedron, and the larger value indicates the higher deviation from the ideal geometry. The obtained value of the eight-coordinated square antiprism (SAPR-8, $D_{4d}$) for $HoW_{10}$ is well below 0.1, characteristic of systems that are only slightly distorted from the ideal symmetry of $D_{4d}$. This is true if we compare the crystallographic coordination sphere with SHAPE's internally defined $D_{4d}$ polyhedron, which is defined with all vertices equidistant to the geometric centre and all edges of the same length ($S(Q,P) = 0.059$), and also if we compare the crystallographic coordination sphere with its $D_{4d}$ idealization ($S(Q,P) = 0.038$).

TABLE S1. The dihedral and axial distortions (from the ideal $D_{4d}$ symmetry) for the $HoW_{10}$ molecules.

| 100 K | | 150 K | | 200 K | |
|---|---|---|---|---|---|
| $\theta$ (°) | $\lvert\theta-45\rvert$ (°) | $\theta$ (°) | $\lvert\theta-45\rvert$ (°) | $\theta$ (°) | $\lvert\theta-45\rvert$ (°) |
| 42.94(65) | 2.06(65) | 42.50(58) | 2.50(58) | 42.85(62) | 2.15(62) |
| 46.93(67) | 1.93(67) | 47.28(64) | 2.28(64) | 47.25(65) | 2.25(65) |
| 47.53(77) | 2.53(77) | 47.42(67) | 2.42(67) | 42.33(74) | 2.33(74) |
| 42.69(79) | 2.31(79) | 42.86(72) | 2.14(72) | 42.66(78) | 2.34(78) |

| 100 K | 150 K | 200 K |
|---|---|---|
| Off-centre distance ($h$ and $h'$) | Off-centre distance ($h$ and $h'$) | Off-centre distance ($h$ and $h'$) |
| 1.218(13) Å | 1.273(11) Å | 1.227(12) Å |
| 1.260(13) Å | 1.223(12) Å | 1.274(12) Å |
| $d = (h - h')/2$ | $d = (h - h')/2$ | $d = (h - h')/2$ |
| 0.021(13) Å | 0.025(11) Å | 0.024(12) Å |

## III. $E$-FIELD INDUCED ESR FREQUENCY SHIFT DUE TO THE TETRAGONAL ANISOTROPY, THE HYPERFINE INTERACTION AND THE ELECTRONIC GYROMAGNETIC RATIO

At each of the experimental frequencies (9.15, 9.45 and 9.88 GHz), the $E$-field-induced shift in the ESR frequency ($\delta f$) is tuned by the changes in $B_4^4$, $A$ and $g_e$ differently. (The sixth order tetragonal transverse anisotropy, $B_6^4$, is also likely to be present, but it has the same effect on the clock transition as $B_4^4$ so we consider only $B_4^4$ here.) This can be understood from Fig. S2a, where the field dependence of the ESR transitions shows significant non-linear behaviour, indicating neither $m_J$ nor $m_I$ is a good quantum number in this field region and the eigenfunctions of the states associated with a given ESR transition are strongly affected by the magnetic field and/or the transition frequency. In order to parameterise the $\delta f$ with the $E$-field-induced changes in the spin Hamiltonian parameters, we performed numerical simulations to analyse the experimental results.

We first consider $\delta f$ at the clock transitions ($f = 9.15$ GHz). Fig. S3a-c show $\delta f$ as a function of small variations in $B_4^4$, $A$ and $g_e$, each varied by $10^{-4}$ of its value in the absence of an $E$-field. We also consider the effect of small errors in the magnetic field since the eigenstate of the $HoW_{10}$ molecule varies with field rapidly around the clock transitions. At the exact clock transition field ($H_{\text{clock}}$), the ESR frequency is immune to small perturbations in the magnetic field ($H$). This is confirmed by the simulation in Fig. S3c, where $\delta f$ is insensitive to changes in the $g$ factor ($\delta g$) (the

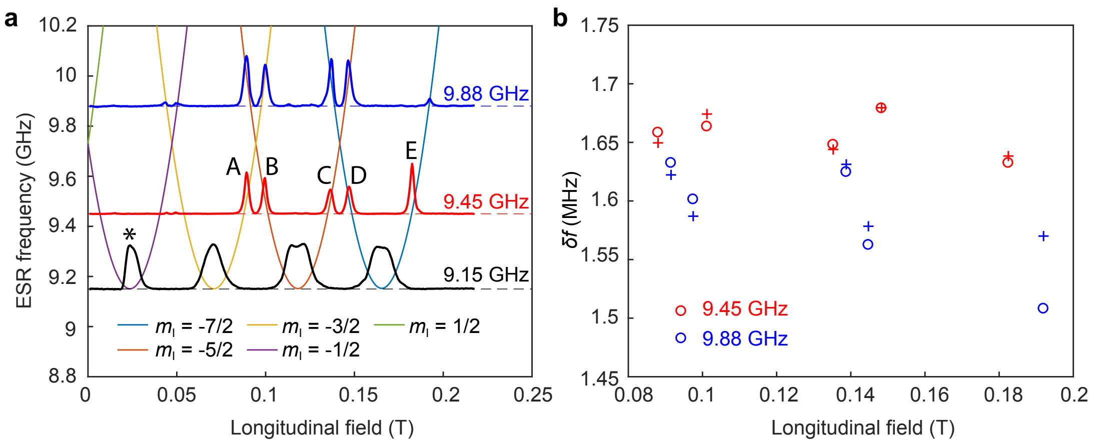


FIG. S2. (a) The ESR transition frequency versus the longitudinal component of the applied magnetic field ($= B_0 \cos 38°$). The ESR spectra are overlayed on top to illustrate the $m_I$ and $\Delta m_J$ value associated with different peaks. The experimental (∘) and simulated (+) $E$-field induced ESR frequency shifts. The measurements were performed at the orientation with the strongest SEC and a fixed $V = 300$ V. The simulation is performed with the parameters in this section.

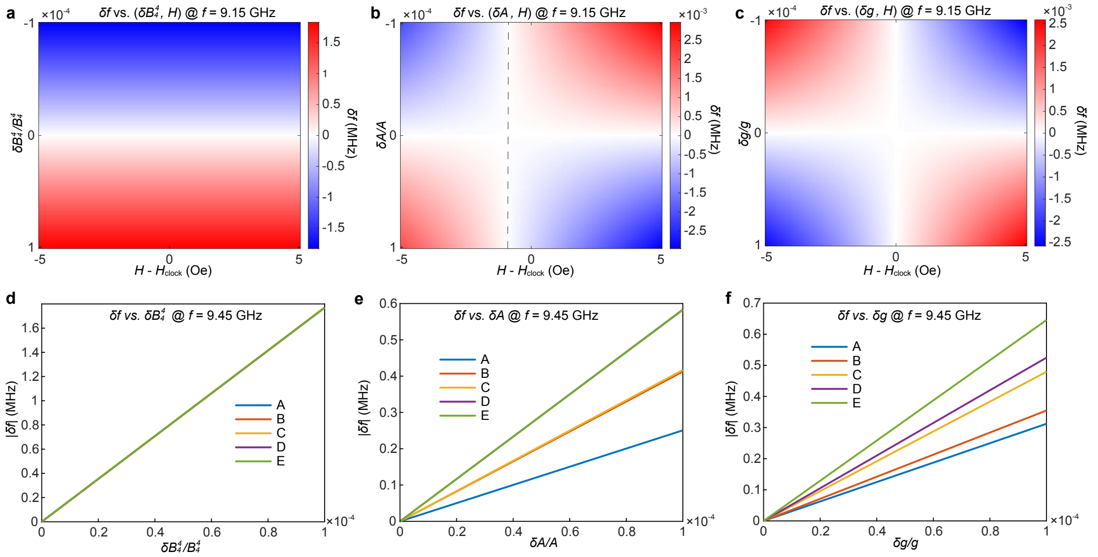


FIG. S3. (a)-(c) 2D colour plots showing the shift in the clock transition frequency (at $f = 9.15$ GHz) as a function of the longitudinal magnetic field and the spin Hamiltonian parameters $B_4^4$, $A$ and $g$. The simulations were performed at the clock transition with the lowest magnetic field [labeled by * in Fig. S2(a)]. The parameters were varied by $10^{-4}$ of their $E = 0$ values (i.e. $|\delta B_4^4/B_4^4| \leq 10^{-4}$) to mimic the $E$-field induced small ESR shift, and the magnetic field was swept by 10 Oe around the clock transition field ($H_{\text{clock}}$) to evaluate the magnetic field dependence. Note the different scales for the colourbars. The frequency shifts induced by $\delta A$ and $\delta g$ are approximately 1000 times weaker than that caused by $\delta B_4^4$ at the clock transition frequency. (d)-(f) Magnetic field dependence for the shift in the ESR frequency (at $f = 9.45$ GHz) as a function of small changes in$B_4^4$, $A$ and $g$. The frequency for all the ESR transitions [transitions labelled as A-E in Fig. S2(a)] exhibits linear dependence for small changes in the parameters. In addition, all A-E transitions show almost identical dependence on small changes in $B_4^4$, hence the five lines appear overlapping in Fig. S2(d).

magnetic field couples to the spins via $\mu_B \mu_0 H g J$, therefore a change in $g$ is equivalent to a change in $H$). Away from the clock transition field, $\delta f$ shows a weak linear dependence on $\delta g$. A similar behaviour was found for $A$, even though the "clock field for hyperfine coupling" (the dashed vertical line in Fig. S3b) is slightly different from $H_{\text{clock}}$ by about 1 Oe. Nevertheless, $\delta f$ is only weakly affected by $\delta A$ or $\delta g$ around the clock transitions. Fig. S3b and c show that by varying $\delta A/A$ or $\delta g/g$ by up to $10^{-4}$, $\delta f$ is changed by less than $3 \times 10^{-3}$ MHz, taking into account the possibility of errors in the applied magnetic field. In fact, in order to generate a $\delta f$ of several MHz, a $\delta A/A$ ($\delta g/g$) $\approx 10\%$ is required, which is unlikely for the $E$-field applied in experiments. By contrast, a strong linear dependence for $\delta B_4^4$

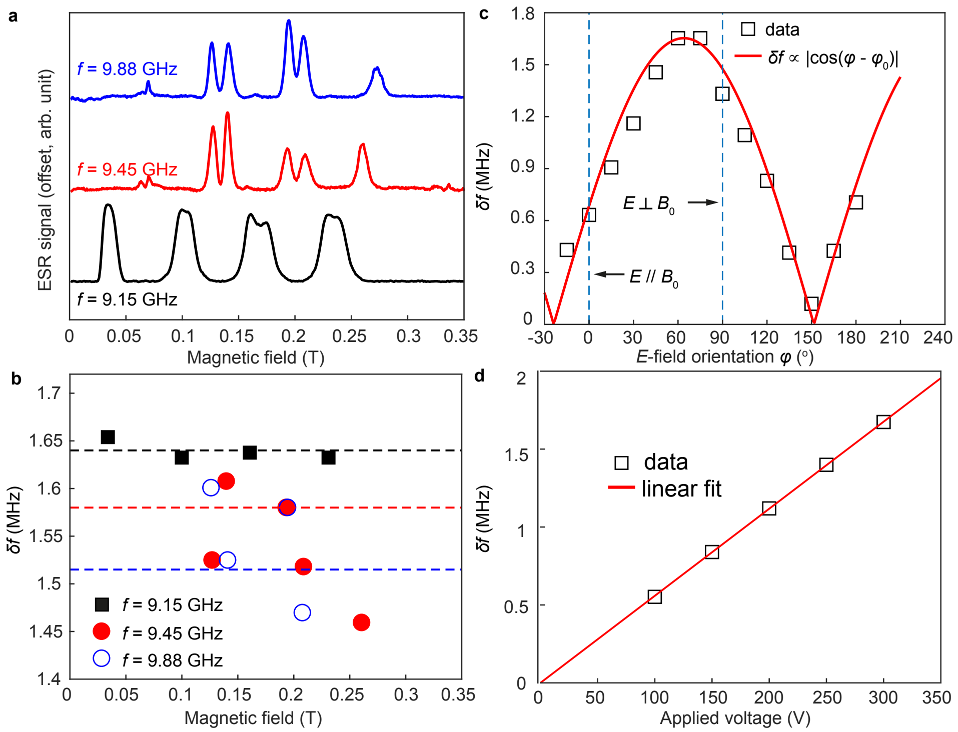


FIG. S4. Data recorded on Crystal B. (a) ESR spectra recorded at the CT frequency (9.15 GHz) and elevated frequencies (9.45 and 9.88 GHz). (b) shows the $E$-field effected measured on the corresponding transitions. The electric field is applied in the orientation with the strongest SEC. (c) Orientation dependence of the $E$-field induced frequency shift. The data were obtained with $f = 9.15$ GHz, $V = 300$ V and $B_0 = 0.0338$ T. (d) The frequency shift (recorded with $f = 9.15$ GHz and $B_0 = 0.0338$ T) versus the applied voltage showing a linear $E$-field coupling in Crystal B.

was found and this relation is insensitive to small errors in the magnetic field (Fig. S3a). In addition, the numerical simulation gives almost identical $\delta f$ versus $\delta B_4^4$ relations for all four clock transitions (not shown), which is consistent with the experimental results that $\delta f$ is magnetic field independent at the clock transition frequency (Fig.2d in the main text).

At elevated frequencies, $\delta f$ is exhibits comparable linear dependence on $\delta B_4^4$, $\delta A$ and $\delta g$. Fig. S3d-f show the simulation performed at $f = 9.45$ GHz for the different ESR transitions labeled in Fig S2a. While $\delta f$ versus $\delta B_4^4$ is almost identical for all the five observed transitions (Fig. S3d), $\delta f$ versus $\delta A$ (and $\delta f$ versus $\delta g$) varies significantly between them. By contrast, the difference between $\delta f$ for A-E transitions at 9.45 GHz is less than 0.1 MHz in our experiments. Therefore, we attribute the $E$-field-induced effect mainly due a modification to the $B_4^4$ parameter, while the effects on $A$ and $g$ are much weaker, i.e. $\delta B_4^4/B_4^4 \gg \delta A/A$ or $\delta g/g$.

The best simulation of $\delta f$ is shown in Fig. S2(b). This is obtained with $\delta B_4^4 = 8.8 \times 10^{-3}$ MHz, $\delta g_e = 1.87 \times 10^{-5}$ and $\delta A = 1.54 \times 10^{-2}$ MHz. As shown in Fig. S2(b), these parameters simulate the fluctuations in $\delta f$ well, except at the highest field resonance observed for $f = 9.88$ GHz. This deviation is likely to be due to the misalignment in the $B_0$ field, which leads to a nontrivial contribution to the ESR transition frequencies due to the transverse component of the magnetic field. Thus the tetragonal transverse anisotropy is the spin Hamiltonian term most strongly coupled to the $E$-field, with $\delta B_4^4/B_4^4 = 9.3 \times 10^{-5}$, compared to $\delta g_e/g_e = 1.6 \times 10^{-5}$ and $\delta A/A = 1.8 \times 10^{-5}$, for an applied voltage of 300 V.

## IV. DATA FROM THE SECOND CRYSTAL

We repeated the experiments on a different crystal, namely Crystal B. Crystal B was picked from a different batch of crystals grown under the same conditions. The ESR spectra [Fig. S4(a)] for Crystal B suggest its easy axis is aligned approximately 45° away from the $B_0$ field.

As shown in Fig. S4, the data recorded on Crystal B are similar to those presented in the main text. In particular, the maximum SEC parameter (11.2 Hz/V m$^{-1}$) is virtually identical to the value reported in the main text (11.4 Hz/V m$^{-1}$). On the other hand, the orientation dependence for Crystal B is offset by approximately 90° compared

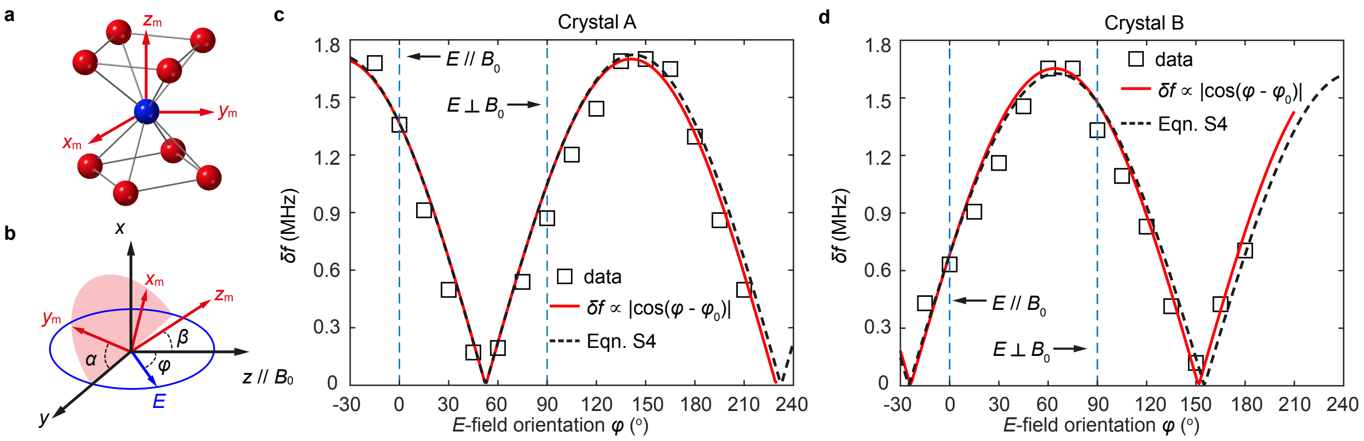


FIG. S5. (a) The molecular frame $(x_{\rm m}, y_{\rm m}, z_{\rm m})$ and (b) the conversion between the molecular and the laboratory frame ($x$, $y$ and $z$). The molecular easy axis, $z_{\rm m}$, lies in the laboratory $x$ – $z$ plane. $\beta$ corresponds to the misalignment between the molecular easy axis and $B_0$ whereas $\alpha$ is unknown. $\varphi$ indicates the orientation of the $E$-field in the $y$ – $z$ plane. (c) and (d) are the orientation dependence data for Crystals A and B, respectively. The dashed lines are the simulations performed with Eqn. S4 and the parameters included in this section.

to the result in the main text. This is due to the crystallographic packing of the $HoW_{10}$ crystals, where the molecular easy axis does not align with any unit cell axes or crystal facets, as well as the limitation that we can only perform a single-axis rotation on the sample. Therefore, it is challenging to control the orientation of the sample in the experiments. We analyse this offset in the next section. Nevertheless, $\delta f$ also follows $\delta f \propto |\cos(\varphi - \varphi_0)|$ in Crystal B with the maximum/minimum of the SEC occurring shifted away from the molecular magnetic axes. Both observations are in agreement with the results on Crystal A described in the main text.

## V. ORIENTATION DEPENDENCE OF THE $E$-FIELD INDUCED FREQUENCY SHIFT

In the $E$-field orientation dependence experiments, the applied electric field is rotated within the laboratory $y$–$z$ plane such that $\mathbf{E} = (0, E\sin\varphi, E\cos\varphi)$. As described in the main text, the frequency shifts for the two inversion-related $HoW_{10}$ subpopulations are opposite. Therefore, the observed $\delta f \propto |\cos(\varphi - \varphi_0)|$ relation implies that for a given $HoW_{10}$ molecule,

$$\begin{aligned} \delta f &= \text{const} \times E\cos(\varphi - \varphi_0) \\ &= \text{const} \times (\cos\varphi_0 E\cos\varphi + \sin\varphi_0 E\sin\varphi) \\ &= \mathbf{A}_l^{\rm E} \cdot \mathbf{E}, \end{aligned} \tag{S1}$$

where $\mathbf{A}_l^{\rm E}$ is the vector depicting the SEC for $HoW_{10}$ molecules is in the laboratory frame. $\mathbf{A}_l^{\rm E}$ is different for Crystals A and B due to the difference in the crystal alignments. In the molecular frame, we define the local coordination $x_{\rm m}$, $y_{\rm m}$ and $z_{\rm m}$, with $z_{\rm m}$ being parallel to the molecular easy axis (Fig. S5a). In this local frame, the SEC coupling $\mathbf{A}_m^{\rm E} = (A_{m,x}, A_{m,y}, A_{m,z})$. We note $\mathbf{A}_m^{\rm E}$ is also affected by the ESR frequency. However, for the low-field CT measured in the orientation dependence experiments, $\delta f$ is only affected by the change in the tetragonal anisotropy, i.e. $\delta B_4^4$, and insensitive to $B_0$ misalignment (as shown in the previous section); therefore, $\mathbf{A}_m^{\rm E}$ is identical for both crystals. Importantly, $\mathbf{A}_m^{\rm E}$ does not coincide with the molecular easy axis, i.e. $A_{m,x} \neq 0$ (and/or $A_{y,m} \neq 0$). This would imply that $\delta f = 0$ when the $E$-field is applied within the molecular hard plane ($\varphi = 90°$), which contradicts with the experimental results.

The conversion between the molecular and the laboratory frame is shown in Fig. S5b and can be described by the rotation matrix $R_m^l$ where

$$R_m^l = \begin{pmatrix} \cos\alpha\cos\beta & -\sin\alpha & -\cos\alpha\sin\beta \\ \sin\alpha\cos\beta & \cos\alpha & -\sin\alpha\sin\beta \\ \sin\beta & 0 & \cos\beta \end{pmatrix} \tag{S2}$$

The $E$-field induced frequency shift:

$$\begin{aligned}\delta f =& \mathbf{A}^{\mathrm{E}}_m \cdot R^l_m \cdot \mathbf{E} \\ =& E(A_{m,y}\cos\alpha - A_{m,x}\sin\alpha)\sin\varphi + E(A_{m,z}\cos\beta - A_{m,x}\cos\alpha\sin\beta - A_{m,y}\sin\alpha\sin\beta)\cos\varphi.\end{aligned} \tag{S3}$$

Without loss of generality, we can choose $x_{\mathrm{m}}$ such that $\mathbf{A}^{\mathrm{E}}_m$ lies in the $x_{\mathrm{m}}$–$z_{\mathrm{m}}$ plane, i.e., $A_{m,x} \neq 0$ and $A_{m,y} = 0$. Eqn. S3 can be further simplified so that

$$\delta f = -EA_{m,x}\sin\alpha\sin\varphi + E(A_{m,z}\cos\beta - A_{m,x}\cos\alpha\sin\beta)\cos\varphi, \tag{S4}$$

where $\beta = 38°$ and $45°$ for crystal A and B, respectively. On the other hand, the angle $\alpha$ *cannot* be directly extrapolated from the ESR spectra. It is the different combinations of $\alpha$ and $\beta$ leads to the non-identical orientation dependence for Crystals A and B, even when the electric field is applied parallel to $B_0$.

The parameters in Eqn. S4 can be calculated using the orientation dependence data. We consider the $E$-field induced frequency shift at $\varphi = 0$ and $90°$ for Crystals A and B. This gives

$$\begin{aligned}\delta f_{\mathrm{A}}(\varphi = 0) =& E(A_{m,z}\cos\beta_{\mathrm{A}} - A_{m,x}\cos\alpha_{\mathrm{A}}\sin\beta_{\mathrm{A}}) \\ \delta f_{\mathrm{A}}(\varphi = 90°) =& -EA_{m,x}\sin\alpha_{\mathrm{A}} \\ \delta f_{\mathrm{B}}(\varphi = 0) =& E(A_{m,z}\cos\beta_{\mathrm{B}} - A_{m,x}\cos\alpha_{\mathrm{B}}\sin\beta_{\mathrm{B}}) \\ \delta f_{\mathrm{B}}(\varphi = 90°) =& -EA_{m,x}\sin\alpha_{\mathrm{B}},\end{aligned} \tag{S5}$$

where the subscript A and B correspond to Crystal A and B, respectively. $\beta_{\mathrm{A}} = 38°$ and $\beta_{\mathrm{B}} = 45°$. $E = 1.5\times10^5$ V/m.

It is worth noting that the sign for $\delta f(\varphi)$ cannot be determined from the experiments. However, based on the orientation dependence, $\delta f_{\mathrm{A}}(\varphi = 0)$ and $\delta f_{\mathrm{A}}(\varphi = 90°)$ should have opposite sign while $\delta f_{\mathrm{B}}(\varphi = 0)$ and $\delta f_{\mathrm{B}}(\varphi = 90°)$ should have the same sign. The exact sign for $\delta f(\varphi)$ is not important as it can be altered by a trivial inversion operation.

The orientation dependence for both crystals can be explained best (Fig. S5c and d) with $A_{m,x} = 9.8$ Hz/(V m$^{-1}$), $A_{m,z} = 6.1$ Hz/(V m$^{-1}$), $\alpha_{\mathrm{A}} = -45°$ and $\alpha_{\mathrm{B}} = 88°$. The analysis shows that the principal SEC axis for $HoW_{10}$ is significantly tilted ($\approx 58°$) away from the molecular easy axis.

## VI. E-FIELD ENABLED SELECTIVE SPIN EXCITATION DATA

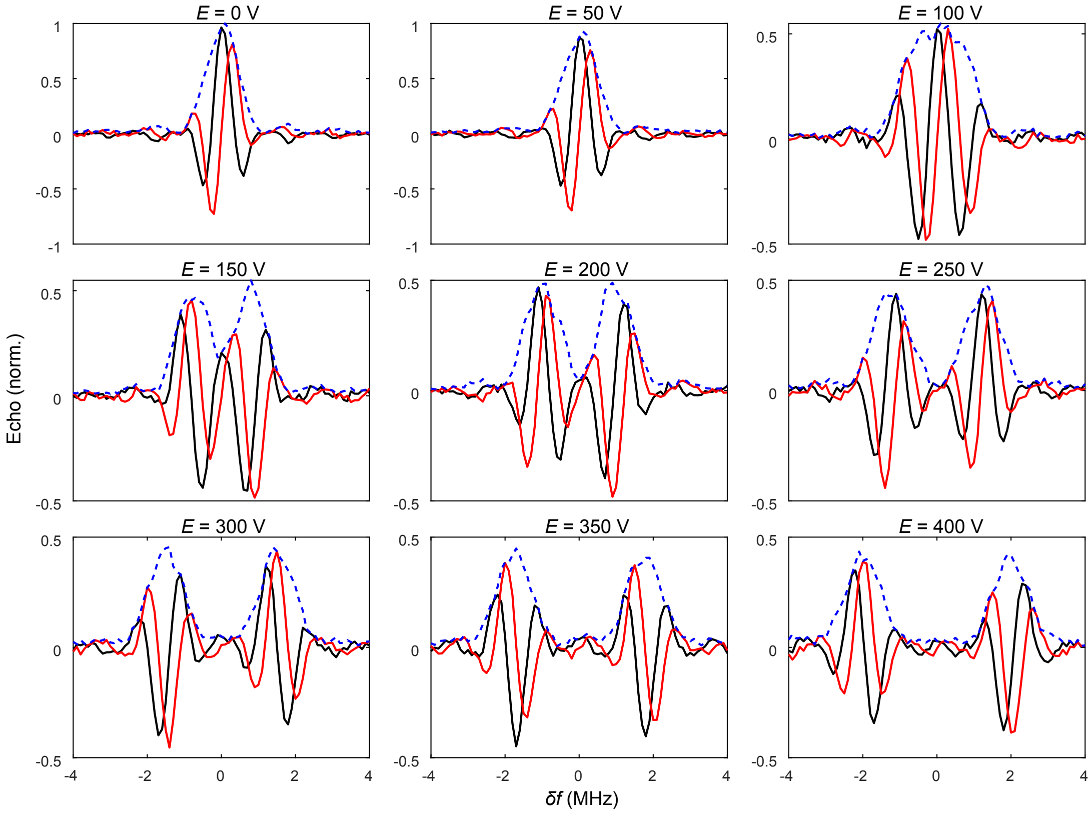


FIG. S6. The spin echo signals versus the frequency shift of the refocusing pulse in the $E$-field-enabled selective spin excitation experiment (Fig. 3 in the main text). Each subplot corresponds to the data recorded with a different applied voltage. The black and red solid lines represent the in-phase and quadrature components respectively and the blue dashed lines represent the absolute magnitude of the spin echo.

## VII. ELECTRIC FIELD EXCITATION FOR SPIN TRANSITIONS

The experiments in this work demonstrate non-resonant coherent spin control with an $E$-field [S3]. However, it is also possible to excite a spin transition with a high-frequency resonant $E$-field. Here we discuss the $E$-field strength required for such operations in $HoW_{10}$. We consider the SEC for the tetragonal anisotropy since it is the dominant contribution in the vicinity of the clock transitions (CT). The application of an oscillating electric field $\boldsymbol{E}(t) = E\cos\omega t$ gives rise to a time dependent term $\delta B_4^4 \hat{O}_4^4 \cos\omega t$, where $\delta B_4^4$ is determined by the amplitude and orientation of the applied $E$-field. This could drive a transition between two spin states, namely $|n\rangle$ and $|m\rangle$, with a transition rate, i.e. Rabi frequency $f_{\text{Rabi}}$, given by

$$hf_{\text{Rabi}} = |\delta B_4^4 \langle m| \hat{O}_4^4 |n\rangle|. \tag{S6}$$

where $h$ is Planck's constant.

Fig. S7 shows the transition rates for the ground $m_J = \pm 4$ multiplet. Exactly at the CT field, the states are eigenfunctions of $\hat{O}_4^4$ and the transition rate vanishes (Fig. S7b). Away from the CT field, an oscillating $B_4^4 \hat{O}_4^4$ term connects states with the same nuclear spin projection $m_I$, allowing an oscillating $E$-field to drive a spin transition directly. Here we consider a 9.88 GHz $E$-field, at which frequency a $T_2 \approx 1\mu$s was observed at 5 K for samples with 0.1% $HoW_{10}$ concentration.

With the maximum observed SEC coupling of $\delta B_4^4/h = 5.9 \times 10^{-2}$ Hz/Vm$^{-1}$, the $E$-field Rabi rate (Eqn. S6) at 9.88 GHz is estimated to be 1.4 Hz/Vm$^{-1}$. Hence, an $E$-field of $10^6$ V/m = 1 mV/nm is required in order to achieve coherent spin control, $f_{\text{Rabi}} < T_2^{-1}$. Such fields are accessible in nanogaps. In fact, it is possible to generate this

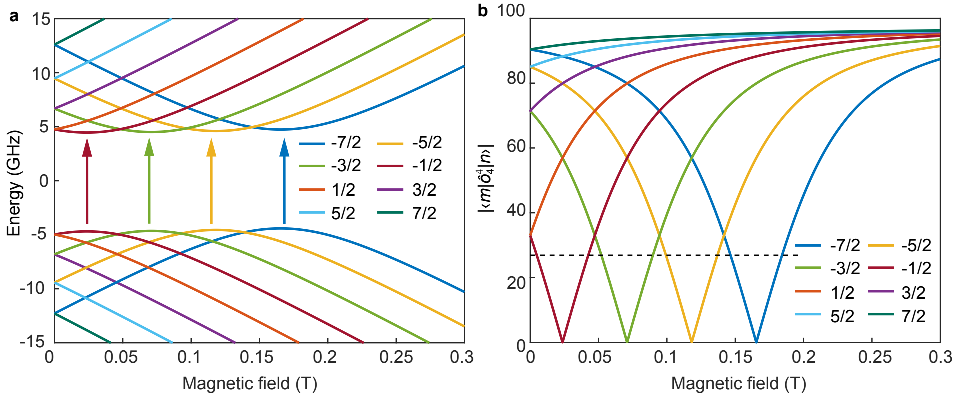


FIG. S7. **a**, The Zeeman energy diagram of the ground $m_J = \pm 4$ multiplet for $HoW_{10}$ with the magnetic field applied parallel to the magnetic axial direction. The states are sorted according to the nuclear spin projection $m_I$. The CTs are indicated by the vertical arrows. **b**, The transition rate for the $E$-field induced spin excitations, $|\langle m|\,\hat{O}_4^4\,|n\rangle|$, between states with the same $m_I$. The horizontal dashed line indicates the transition rate for $f = 9.88$ GHz.

field in certain macroscopic 3D resonators, for instance, a loop-gap resonator [S4], allowing, in principle, ensemble experiments on single-crystal samples.

## VIII. COMPUTATIONAL DETAILS

### A. Electronic and vibrational structure

The time-independent electronic structure was computed using the multireference Complete Active Self-Consistent Field Spin-Orbit (CASSCF-SO) method as implemented in the OpenMOLCAS program package (version 18.09) [S5]. The molecular geometry was extracted from the single-crystal X-ray structure and was fully optimized at density functional theory (DFT) level (*vide infra*). In addition, the electronic structure of the molecular geometry with no prior optimization was calculated. Scalar relativistic effects were taken into account with the Douglas–Kroll–Hess transformation using the relativistically contracted atomic natural orbital ANO-RCC basis set with VDZP quality for all atoms. The active space consisted of 10 electrons on the 7 $f$-orbitals of $Ho^{3+}$ ion. The molecular orbitals were optimized at the CASSCF level in a state-average (SA) over 35 quintets of the ground state term ($L = 6$ for $Ho^{3+}$). The wave functions obtained at CASSCF were then mixed by spin-orbit coupling by means of the RASSI approach. The combined effect of the crystal field and the spin orbit coupling were computed using SINGLE-ANISO module [S6].

The structural optimization of the crystallographic coordinates in vacuum and the vibrational modes calculations were carried out at DFT level using the Gaussian16 package in its revision A.03 [S7]. The vibrational frequency calculations were carried out using both the fully optimized structure and the X-ray crystal structure with no optimization. The PBE0 hybrid exchange-correlation functional was used for both optimization and frequency calculations in combination with Stuttgart RSC ANO basis set with effective core potential (ECP) for the $Ho^{3+}$ cation. CRENBL basis set have been used for W with corresponding ECP potential and 6-31G(d,p) basis set had been used for oxygen. An 'ultra-fine' integration grid and 'very tight' SCF convergence criterion were applied. Dispersion effects were taken into account using the empirical GD3BJ dispersion correction.

The crystalline environment of the polyanion has an effect in its electric dipole. We estimated this effect by recalculating the electric dipole for all the distorted geometries in an embedding consisting in a crystalline fragment. We chose this fragment to consist of 11 units of $HoW_{10}$ molecule, 11× ( $Na_9[Ho(W_5O_{18})_2]\cdot 35H_2O$). The charge analysis of the environment atoms was performed in Gaussian16 using MKUFF uses the Merz-Kollman-Singh approximate charges to fit the electrostatic potential of the molecule. The electronic energy for the central $HoW_{10}$ molecule in the presence of the environment as point-charges was stabilized at same level of DFT as optimization and vibrational frequencies calculations (the input/output files are provided as SI files).

### B. General methodology

Let us start by laying out the effective Hamiltonian we will use to model the spin-electric coupling in $HoW_{10}$. $\hat{H}_{\text{eff}}$ is the sum of (i) a time-independent crystal-field Hamiltonian $\hat{H}_{\text{CF}}(J)$, which is only a function of the equilibrium molecular geometry acting on the ground multiplet $J$ and (ii) the perturbation $\hat{H}_{\text{CF}}(J, Q_{\text{eff}}(V))$ resulting from the collective distortion coordinate $Q_{\text{eff}}(V)$ which is in itself a function of the externally applied electric voltage $V$:

$$\hat{H}_{\text{eff}} = \hat{H}_{\text{CF}}(J) + \hat{H}_{\text{CF}}(J, Q_{\text{eff}}(V)) \tag{S7}$$

In order to estimate the effect of the molecular distortion caused by the external electric field, we chose to decompose such a distortion in the geometrical basis of the vibrational modes. Since we are operating in the regime of very small distortions (small fractions of an angstrom), the total effect of every vibrational normal mode will be additive in a very good approximation. Thus, we proceeded considering that, being $3N - 6$ the number of vibrational modes ($n$) in nonlinear molecules of $N$ atoms and that, for a given applied voltage, the effective distortion $\vec{Q}_{\text{eff}}$ can be written as the additive effect of all of the displacements corresponding to $n$ vibrational modes as defined in Eqn. S8:

$$\vec{Q}_{\text{eff}}(V) = \sum_n Q_{(\text{eff},n)}(V) = Q_{(\text{eff},1)}(V) + Q_{(\text{eff},2)}(V) + \ldots + Q_{(\text{eff},3N-6)}(V) \tag{S8}$$

where $Q_{(\text{eff},n)}(V)$ is the distortion attained by a normal mode $n$ at a given applied potential $V$, which can be further expressed as displacement vector of normal mode as in Eqn. S9:

$$\vec{Q}_{(\text{eff},n)} = v_n(V) \begin{pmatrix} q_{x,n} \\ q_{y,n} \\ q_{z,n} \end{pmatrix} \tag{S9}$$

Thus, the total spin-electric coupling can be effectively estimated if one is able to relate the external voltage with the induced molecular distortions, and these with the perturbation $\hat{H}_{\text{CF}}(J, Q_{\text{eff}}(V))$. In the subsequent sections, we detail, step by step, the general methodology that we employed to estimate the spin-electric coupling in this molecular spin qubit.

### C. Step 1: Derivation of the relation between molecular distortion and electric field

To model the evolution of the tunneling splitting caused by an electrical field, we first had to correlate the distortion of atomic coordinates and the $E$-field. For this we considered the fact that the perturbation caused by applied $E$-field is necessarily at the cost of molecular distortions from a near-equilibrium structure. In particular, a central assumption in our methodology is that the rise in potential energy due to the displacement of the atomic positions – in the form of a harmonic oscillator – is exactly matched by the stabilization of the potential energy due to the change in the molecular electric dipole in presence of an external electric field.

For technical reasons, we could not calculate the effect of an external $E$-field in terms of molecular distortions directly. Instead, we calculated this indirectly using a set of distorted structures following the vibrational modes of $HoW_{10}$ as input and estimated the change in electrical dipole associated to each distortion. Then, the electrical field that is required to achieve a given distortion was estimated by computing the harmonic potential energy and dipole moment at a given point. This was carried out at different points along the vibrational path by using the following Eqn. S10:

$$U_n = -\Delta p E \cos\rho \tag{S10}$$

where $U_n$ is the harmonic potential energy, $\Delta p$ is the increase in the (molecular) electric dipole moment at any given distortion compared with the value in the absence of distortions and $\rho$ is the angle between the external electric field $E$ and the dipole moment. Except where we were explicitly calculating the angular dependence, we worked assuming that the electric field $E$ was applied exactly in the direction of the molecular electric dipole $p$ in the equilibrium geometry. Moreover, since experimentally we worked in the regime of very small distortions, we assumed that the change in the electric dipole $\Delta p$ can be properly approximated at all experimentally relevant voltages by a change in its modulus $|\Delta p|$ and we neglected the effect of any change in the angle $\Delta\rho$ caused by the distortion:

$$E = -\frac{U_n}{|\Delta p|} \tag{S11}$$

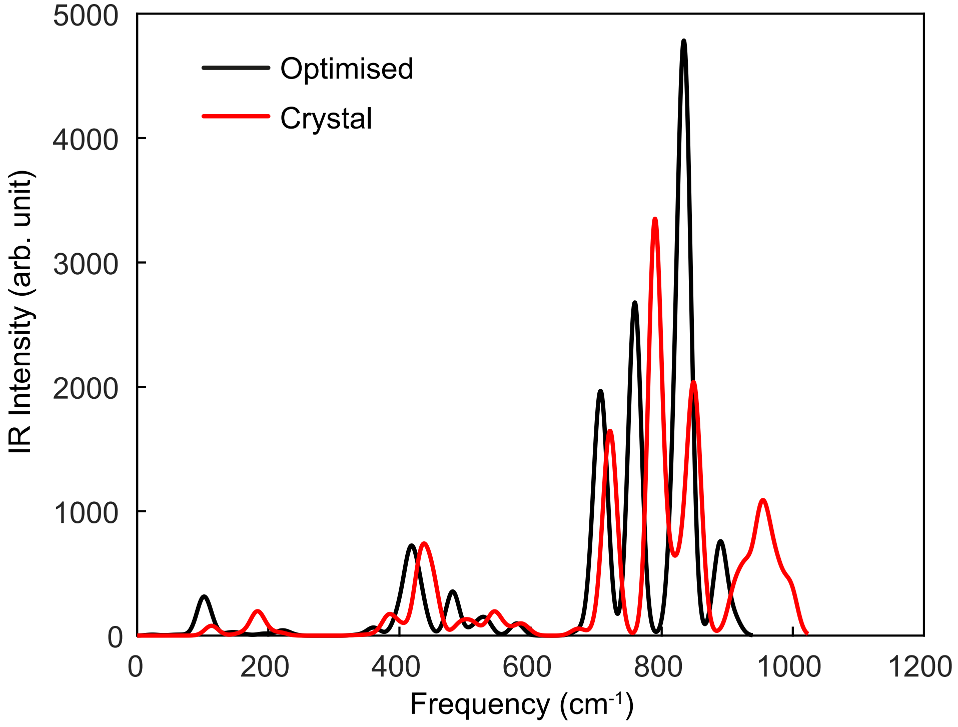


FIG. S8. Harmonic vibrational frequencies for $HoW_{10}$, IR intensities with Gaussian-convoluted FWHM of 10 $cm^{-1}$ for optimized structure (black) and for crystal structure (red).

Following this approach, firstly we calculated the potential energy for a given vibrational mode $n$ by using the classical potential energy Eqn. S12:

$$U_n = \frac{1}{2} k_n Q_n^2 \tag{S12}$$

where $k_n$ is the force constant of mode $n$ and $Q_n$ is a displacement along the vibrational coordinate $\vec{Q}_n$ of mode $n$. We choose the origin of potential energy $U_n = 0$ at the equilibrium coordinates $\vec{Q}_{\mathrm{eq}}$ where $v_n = 0$.

We then defined for each normal mode a series of displacement vectors of increasing moduli, given by

$$\vec{Q}_n = v_n \begin{pmatrix} q_{n,x} \\ q_{n,y} \\ q_{n,z} \end{pmatrix} \tag{S13}$$

with the corresponding series distorted atomic coordinates being given by $\vec{Q}_{\mathrm{dist}} = \vec{Q}_{\mathrm{eq}} + \vec{Q}_n$ where '$v_n$' is a scalar multiplier which defines the step or modulus of the displacement between consecutive distorted geometries following a given vibrational path. The value of $v_n$ was chosen to be large enough to produce consistent values of the electric dipole, since distortions corresponding to the experimentally realistic perturbations are very small and we found that the results were heavily affected by numerical errors in the Gaussian output.

At this point, the procedure is straightforward. The external electric field $E$ is the result of an externally applied voltage $V_{\mathrm{ext}}$, with the relation between the two magnitudes being given by the distance $d = 0.002$ m between two plates:

$$E = V_{\mathrm{ext}}/d \tag{S14}$$

At each of the same set of distorted coordinates where we calculated the elastic distortion energy as detailed above, we also computed the dipole moment at the DFT level. The external voltage $V$ resulting in an electric field that achieves an energy match between the molecular distortion energy $Q$ cost and the electric potential energy stabilization is the external voltage required for precisely that degree of molecular distortion $Q_{(\mathrm{eff},n)}(V)$ . Again, note that the useful information we can get for changes in the electrical dipole is limited by numerical noise for distortions below a certain threshold; we therefore needed to apply relatively large distortions (larger than 0.02 Å). The electric field

needed to achieve any given molecular distortion is given by combining Eqn. S14 and S12, i.e. the electric field where the stabilization due to the change in the electric dipole potential energy is exactly enough to compensate the cost in terms of elastic spring energy. Due to the above mentioned technical limitations, the theoretically obtained distortions are relatively large, corresponding to electric fields that are approximately 5 orders of magnitude above the experimentally available $E$-field. As discussed below, we performed a quadratic interpolation to the limit of small distortions to access the experimentally relevant electric fields.

### D. Step 2: DFT calculation of vibrational spectrum and electric dipoles

The obtained frequencies for optimized- and crystal-geometry are provided in Table S2 and S3 respectively, and also plotted in Fig. S8. From Fig. S8, we observed the vibrational frequency for optimized geometry is redshifted with respect to crystal geometry. Further, we analysed that the IR-active mode in both cases; they present similar displacement patterns. (Output files are provided for analysis of displacement pattern.) This gives us confidence to use the optimized geometry for further analysis.

TABLE S2: Frequencies ( $cm^{-1}$) computed at the DFT level for relaxed-geometry, resultant displacement $d_{\mathrm{Ho}}$ (Å), IR/k and effective normalized displacement $Q_{(\mathrm{eff},n)}$ for each normal mode (n).

| Mode ($n$) | Frequency ($cm^{-1}$) | $d_{\mathrm{Ho}}$ (Å) | IR/k $\left(\frac{\mathrm{km.mol}^{-1}}{\mathrm{mDyne.Å}^{-1}}\right)$ | $\left\lvert Q_{(\mathrm{eff},n)}\right\rvert$ (300V) ($10^{-5}\times$Å) |
|---|---|---|---|---|
| 1 | 8.62 | 0.008 | 5.22 | 6.6608 |
| 2 | 17.94 | 0.022 | 200.69 | 7.4497 |
| 3 | 18.43 | 0.004 | 102.42 | 10.7773 |
| 4 | 24.33 | 0.072 | 493.41 | 3.6713 |
| 5 | 29.97 | 0.046 | 0.68 | 0.0995 |
| 6 | 43.22 | 0.169 | 5.39 | 0.6575 |
| 7 | 54.02 | 0.501 | 25.52 | 1.1618 |
| 8 | 58.39 | 0.304 | 13.89 | 0.8202 |
| 9 | 67.12 | 0.302 | 11.34 | 1.0228 |
| 10 | 70.95 | 0.433 | 16.91 | 0.4642 |
| 11 | 99.61 | 0.481 | 611.40 | 0.0389 |
| 12 | 106.52 | 0.070 | 0.54 | 0.0221 |
| 13 | 106.78 | 0.112 | 6.77 | 0.0461 |
| 14 | 107.26 | 0.089 | 0.58 | 0.4116 |
| 15 | 108.76 | 0.223 | 470.90 | 0.0632 |
| 16 | 114.68 | 0.028 | 0.28 | 0.0410 |
| 17 | 114.71 | 0.036 | 1.44 | 0.1167 |
| 18 | 140.11 | 0.054 | 4.85 | 0.1636 |
| 19 | 140.76 | 0.021 | 1.24 | 0.0325 |
| 20 | 141.19 | 0.027 | 1.21 | 0.1342 |
| 21 | 142.11 | 0.007 | 0.04 | 0.0886 |
| 22 | 143.98 | 0.126 | 24.44 | 0.0272 |
| 23 | 144.75 | 0.032 | 0.01 | 0.0311 |
| 24 | 157.60 | 0.018 | 5.09 | 0.1569 |
| 25 | 158.17 | 0.002 | 0.00 | 0.0017 |
| 26 | 159.14 | 0.007 | 0.78 | 0.0161 |
| 27 | 159.88 | 0.047 | 11.82 | 0.0915 |
| 28 | 160.56 | 0.038 | 10.16 | 0.3349 |
| 29 | 161.30 | 0.001 | 0.01 | 0.0428 |
| 30 | 167.76 | 0.002 | 0.01 | 0.0116 |
| 31 | 167.77 | 0.002 | 0.01 | 0.0104 |
| 32 | 184.62 | 0.006 | 0.11 | 0.0521 |
| 33 | 184.73 | 0.005 | 0.06 | 0.0656 |
| 34 | 193.02 | 0.052 | 28.11 | 0.0565 |
| 35 | 202.14 | 0.012 | 0.02 | 0.0964 |
| 36 | 216.40 | 0.001 | 1.60 | 0.1246 |
| 37 | 216.89 | 0.003 | 2.39 | 0.1896 |
| 38 | 218.12 | 0.001 | 0.62 | 0.0411 |
| 39 | 218.13 | 0.002 | 0.85 | 0.0340 |
| 40 | 218.22 | 0.002 | 0.41 | 0.0240 |
| 41 | 218.24 | 0.003 | 0.82 | 0.0312 |
| 42 | 219.96 | 0.006 | 26.18 | 0.2854 |

| | | | | |
|---|---|---|---|---|
| 43 | 220.00 | 0.006 | 29.47 | 0.2012 |
| 44 | 220.07 | 0.004 | 5.10 | 0.0094 |
| 45 | 220.47 | 0.001 | 0.19 | 0.0295 |
| 46 | 223.18 | 0.002 | 2.87 | 0.0788 |
| 47 | 224.41 | 0.005 | 0.69 | 0.0797 |
| 48 | 230.85 | 0.000 | 10.81 | 0.1760 |
| 49 | 231.24 | 0.001 | 11.22 | 0.1345 |
| 50 | 231.75 | 0.000 | 0.39 | 0.0506 |
| 51 | 232.10 | 0.001 | 0.52 | 0.0578 |
| 52 | 235.13 | 0.000 | 0.10 | 0.0101 |
| 53 | 235.33 | 0.000 | 0.01 | 0.0082 |
| 54 | 257.49 | 0.001 | 0.00 | 0.0079 |
| 55 | 257.49 | 0.001 | 0.00 | 0.0075 |
| 56 | 289.55 | 0.001 | 0.00 | 0.0165 |
| 57 | 291.07 | 0.001 | 0.00 | 0.0096 |
| 58 | 329.19 | 0.002 | 0.04 | 0.0120 |
| 59 | 329.25 | 0.002 | 0.05 | 0.0083 |
| 60 | 337.26 | 0.015 | 2.36 | 0.1373 |
| 61 | 337.36 | 0.007 | 0.65 | 0.0500 |
| 62 | 337.40 | 0.015 | 2.31 | 0.0362 |
| 63 | 337.72 | 0.007 | 0.49 | 0.0084 |
| 64 | 351.19 | 0.011 | 0.08 | 0.0187 |
| 65 | 354.95 | 0.000 | 0.03 | 0.0372 |
| 66 | 355.21 | 0.002 | 0.22 | 0.0298 |
| 67 | 359.02 | 0.016 | 15.44 | 0.1602 |
| 68 | 360.26 | 0.022 | 24.79 | 0.2391 |
| 69 | 363.49 | 0.016 | 9.62 | 0.0729 |
| 70 | 399.03 | 0.002 | 69.09 | 0.0082 |
| 71 | 399.78 | 0.003 | 19.05 | 0.0852 |
| 72 | 399.80 | 0.002 | 6.49 | 0.0649 |
| 73 | 404.19 | 0.005 | 0.34 | 0.0049 |
| 74 | 414.55 | 0.004 | 28.49 | 0.1228 |
| 75 | 414.92 | 0.003 | 25.14 | 0.2106 |
| 76 | 416.67 | 0.008 | 110.35 | 0.3117 |
| 77 | 416.90 | 0.008 | 106.28 | 0.3797 |
| 78 | 417.53 | 0.004 | 23.52 | 0.0566 |
| 79 | 417.69 | 0.004 | 26.77 | 0.1741 |
| 80 | 429.95 | 0.010 | 120.59 | 0.0066 |
| 81 | 431.15 | 0.006 | 5.73 | 0.0902 |
| 82 | 435.19 | 0.003 | 0.16 | 0.0161 |
| 83 | 436.31 | 0.009 | 1.00 | 0.0101 |
| 84 | 436.72 | 0.006 | 28.09 | 0.0001 |
| 85 | 437.91 | 0.008 | 6.11 | 0.0356 |
| 86 | 479.05 | 0.001 | 0.79 | 0.0230 |
| 87 | 479.34 | 0.001 | 0.61 | 0.0335 |
| 88 | 480.96 | 0.006 | 74.70 | 0.2299 |
| 89 | 481.29 | 0.007 | 76.78 | 0.2741 |
| 90 | 489.34 | 0.000 | 1.05 | 0.0093 |
| 91 | 489.38 | 0.001 | 1.35 | 0.0323 |
| 92 | 514.29 | 0.010 | 23.83 | 0.0278 |
| 93 | 515.09 | 0.001 | 0.32 | 0.0087 |
| 94 | 515.25 | 0.001 | 0.20 | 0.0101 |
| 95 | 516.21 | 0.001 | 0.03 | 0.0237 |
| 96 | 520.31 | 0.002 | 0.24 | 0.0191 |
| 97 | 521.09 | 0.002 | 0.16 | 0.0324 |
| 98 | 528.07 | 0.003 | 4.88 | 0.0163 |
| 99 | 529.22 | 0.003 | 0.17 | 0.0216 |
| 100 | 530.46 | 0.002 | 36.75 | 0.0084 |
| 101 | 531.81 | 0.002 | 4.44 | 0.0169 |
| 102 | 535.59 | 0.002 | 0.23 | 0.0237 |
| 103 | 536.21 | 0.002 | 1.91 | 0.0277 |
| 104 | 554.98 | 0.000 | 0.02 | 0.0075 |
| 105 | 555.04 | 0.000 | 0.02 | 0.0073 |
| 106 | 578.43 | 0.000 | 7.88 | 0.0580 |

| | | | | |
|---|---|---|---|---|
| 107 | 579.04 | 0.000 | 7.57 | 0.0588 |
| 108 | 579.13 | 0.000 | 7.80 | 0.0548 |
| 109 | 579.49 | 0.000 | 6.37 | 0.0650 |
| 110 | 671.58 | 0.001 | 6.78 | 0.0042 |
| 111 | 671.94 | 0.001 | 0.14 | 0.0022 |
| 112 | 697.89 | 0.013 | 49.15 | 0.1883 |
| 113 | 698.02 | 0.014 | 52.43 | 0.0739 |
| 114 | 708.22 | 0.020 | 160.98 | 0.3199 |
| 115 | 708.89 | 0.020 | 165.23 | 0.1571 |
| 116 | 759.02 | 0.005 | 449.21 | 0.0015 |
| 117 | 766.97 | 0.000 | 0.20 | 0.0127 |
| 118 | 819.87 | 0.005 | 123.01 | 0.0038 |
| 119 | 825.83 | 0.000 | 2.13 | 0.0242 |
| 120 | 827.39 | 0.003 | 20.35 | 0.0296 |
| 121 | 829.18 | 0.001 | 21.79 | 0.1111 |
| 122 | 829.87 | 0.003 | 16.64 | 0.0612 |
| 123 | 832.87 | 0.001 | 3.85 | 0.0286 |
| 124 | 835.00 | 0.006 | 207.17 | 0.2909 |
| 125 | 835.25 | 0.005 | 194.49 | 0.1041 |
| 126 | 835.94 | 0.004 | 172.35 | 0.1051 |
| 127 | 885.27 | 0.001 | 13.24 | 0.0278 |
| 128 | 886.09 | 0.001 | 1.52 | 0.0375 |
| 129 | 886.14 | 0.001 | 1.99 | 0.0009 |
| 130 | 887.81 | 0.000 | 0.44 | 0.0294 |
| 131 | 888.08 | 0.001 | 0.92 | 0.0111 |
| 132 | 889.51 | 0.001 | 47.50 | 0.1326 |
| 133 | 891.28 | 0.002 | 31.47 | 0.0579 |
| 134 | 910.99 | 0.005 | 15.48 | 0.0066 |
| 135 | 913.68 | 0.001 | 0.01 | 0.0117 |

TABLE S3: Frequencies ( $cm^{-1}$) computed at the DFT level for crystal-geometry, resultant displacement $d_{\text{Ho}}$ (Å), IR/k and effective normalized displacement $Q_{(\text{eff},n)}$ for each normal mode (n).

| Mode ($n$) | Frequency ($cm^{-1}$) | $d_{\text{Ho}}$ (Å) | IR/k $\left(\frac{\text{km.mol}^{-1}}{\text{mDyne.Å}^{-1}}\right)$ | $\lvert Q_{(\text{eff},n)}\rvert$ (300V) ($10^{-5}\times$Å) |
|---|---|---|---|---|
| 1 | -28.79 | 0.003 | 0.07 | 1.5949 |
| 2 | -15.56 | 0.165 | 1.94 | 5.9928 |
| 3 | -9.24 | 0.167 | 4.84 | 57.8133 |
| 4 | 50.80 | 0.005 | 0.02 | 0.0312 |
| 5 | 58.62 | 0.015 | 1.53 | 0.2590 |
| 6 | 59.16 | 0.017 | 0.98 | 0.2560 |
| 7 | 89.61 | 0.014 | 0.45 | 0.0228 |
| 8 | 93.12 | 0.029 | 0.24 | 0.3186 |
| 9 | 107.58 | 0.355 | 1.20 | 0.1921 |
| 10 | 108.82 | 0.382 | 0.52 | 0.0847 |
| 11 | 112.86 | 0.385 | 165.61 | 0.0132 |
| 12 | 116.50 | 0.180 | 17.97 | 0.0609 |
| 13 | 120.99 | 0.079 | 4.18 | 0.0342 |
| 14 | 123.78 | 0.067 | 2.63 | 0.1512 |
| 15 | 124.79 | 0.112 | 2.42 | 0.1503 |
| 16 | 127.15 | 0.064 | 0.20 | 0.2250 |
| 17 | 129.14 | 0.090 | 5.90 | 0.0433 |
| 18 | 132.29 | 0.033 | 0.43 | 0.1431 |
| 19 | 140.81 | 0.022 | 0.39 | 0.1992 |
| 20 | 146.08 | 0.044 | 0.62 | 0.1236 |
| 21 | 146.48 | 0.037 | 0.10 | 0.0358 |
| 22 | 148.52 | 0.034 | 0.09 | 0.0097 |
| 23 | 155.17 | 0.201 | 4.19 | 0.1612 |
| 24 | 156.35 | 0.193 | 2.73 | 0.0976 |
| 25 | 157.65 | 0.236 | 10.48 | 0.1913 |
| 26 | 159.42 | 0.093 | 0.71 | 0.1014 |
| 27 | 159.87 | 0.097 | 3.47 | 0.0738 |

| | | | | |
|---|---|---|---|---|
| 28 | 161.39 | 0.056 | 0.50 | 0.0596 |
| 29 | 162.42 | 0.022 | 0.47 | 0.0567 |
| 30 | 163.17 | 0.089 | 2.36 | 0.0599 |
| 31 | 165.24 | 0.065 | 2.98 | 0.0173 |
| 32 | 175.82 | 0.075 | 67.22 | 0.0555 |
| 33 | 179.44 | 0.041 | 30.81 | 0.1789 |
| 34 | 179.75 | 0.067 | 43.34 | 0.0521 |
| 35 | 182.99 | 0.101 | 145.85 | 0.1236 |
| 36 | 184.26 | 0.106 | 160.25 | 0.3455 |
| 37 | 186.40 | 0.012 | 27.90 | 0.4980 |
| 38 | 187.52 | 0.022 | 15.49 | 0.0194 |
| 39 | 192.14 | 0.035 | 21.37 | 0.0162 |
| 40 | 192.96 | 0.006 | 26.53 | 0.3005 |
| 41 | 196.98 | 0.025 | 19.73 | 0.0464 |
| 42 | 199.59 | 0.017 | 5.92 | 0.0470 |
| 43 | 201.54 | 0.038 | 7.69 | 0.1226 |
| 44 | 202.02 | 0.007 | 6.97 | 0.1228 |
| 45 | 203.38 | 0.026 | 6.43 | 0.0787 |
| 46 | 210.95 | 0.010 | 0.45 | 0.0160 |
| 47 | 212.77 | 0.011 | 2.75 | 0.0731 |
| 48 | 215.70 | 0.012 | 13.18 | 0.1985 |
| 49 | 217.91 | 0.009 | 11.12 | 0.0727 |
| 50 | 221.22 | 0.028 | 7.40 | 0.0169 |
| 51 | 223.05 | 0.007 | 1.72 | 0.0656 |
| 52 | 223.32 | 0.003 | 0.20 | 0.0418 |
| 53 | 224.14 | 0.004 | 0.27 | 0.0590 |
| 54 | 248.64 | 0.002 | 0.06 | 0.0078 |
| 55 | 251.92 | 0.002 | 0.05 | 0.0332 |
| 56 | 286.74 | 0.001 | 0.05 | 0.0036 |
| 57 | 298.58 | 0.002 | 0.03 | 0.0087 |
| 58 | 334.12 | 0.007 | 2.02 | 0.0810 |
| 59 | 336.97 | 0.006 | 1.14 | 0.0110 |
| 60 | 340.45 | 0.005 | 0.92 | 0.0008 |
| 61 | 342.15 | 0.004 | 0.39 | 0.0243 |
| 62 | 350.79 | 0.005 | 0.46 | 0.0120 |
| 63 | 357.49 | 0.021 | 3.17 | 0.0321 |
| 64 | 359.96 | 0.019 | 3.38 | 0.0089 |
| 65 | 368.65 | 0.006 | 1.59 | 0.0488 |
| 66 | 370.48 | 0.011 | 2.79 | 0.1127 |
| 67 | 371.56 | 0.008 | 1.56 | 0.0184 |
| 68 | 382.80 | 0.050 | 48.78 | 0.2183 |
| 69 | 384.12 | 0.049 | 52.70 | 0.3082 |
| 70 | 400.93 | 0.016 | 42.42 | 0.0409 |
| 71 | 408.80 | 0.002 | 0.08 | 0.0269 |
| 72 | 410.29 | 0.001 | 0.53 | 0.0145 |
| 73 | 413.73 | 0.006 | 3.38 | 0.0250 |
| 74 | 429.15 | 0.007 | 95.17 | 0.3867 |
| 75 | 430.56 | 0.006 | 33.47 | 0.0083 |
| 76 | 432.50 | 0.008 | 63.87 | 0.1998 |
| 77 | 433.66 | 0.004 | 19.89 | 0.0801 |
| 78 | 436.61 | 0.013 | 115.18 | 0.0278 |
| 79 | 438.18 | 0.002 | 10.90 | 0.0676 |
| 80 | 441.65 | 0.006 | 2.78 | 0.0513 |
| 81 | 446.08 | 0.008 | 42.41 | 0.2545 |
| 82 | 447.02 | 0.003 | 7.58 | 0.0313 |
| 83 | 448.84 | 0.006 | 44.60 | 0.0859 |
| 84 | 452.42 | 0.004 | 49.01 | 0.2869 |
| 85 | 454.07 | 0.004 | 52.70 | 0.1299 |
| 86 | 483.17 | 0.001 | 0.13 | 0.0010 |
| 87 | 485.31 | 0.002 | 1.73 | 0.0224 |
| 88 | 489.00 | 0.004 | 6.81 | 0.0902 |
| 89 | 491.33 | 0.007 | 15.24 | 0.1141 |
| 90 | 494.43 | 0.005 | 6.10 | 0.0415 |
| 91 | 498.30 | 0.005 | 13.19 | 0.0674 |

| | | | | |
|---|---|---|---|---|
| 92 | 509.57 | 0.008 | 29.06 | 0.0556 |
| 93 | 514.27 | 0.002 | 2.15 | 0.0366 |
| 94 | 517.25 | 0.001 | 1.78 | 0.0261 |
| 95 | 519.36 | 0.005 | 6.09 | 0.0886 |
| 96 | 522.59 | 0.002 | 1.27 | 0.0266 |
| 97 | 531.27 | 0.002 | 0.77 | 0.0276 |
| 98 | 538.87 | 0.002 | 14.62 | 0.0416 |
| 99 | 539.62 | 0.002 | 0.24 | 0.0076 |
| 100 | 544.50 | 0.002 | 32.07 | 0.0330 |
| 101 | 547.37 | 0.002 | 17.43 | 0.0345 |
| 102 | 553.72 | 0.002 | 1.18 | 0.0129 |
| 103 | 557.35 | 0.003 | 3.37 | 0.0172 |
| 104 | 560.95 | 0.001 | 3.89 | 0.0681 |
| 105 | 565.08 | 0.002 | 7.64 | 0.0844 |
| 106 | 581.27 | 0.001 | 13.83 | 0.0126 |
| 107 | 587.13 | 0.001 | 8.14 | 0.0209 |
| 108 | 592.71 | 0.001 | 7.74 | 0.0688 |
| 109 | 597.88 | 0.002 | 2.25 | 0.0341 |
| 110 | 668.48 | 0.004 | 6.06 | 0.0727 |
| 111 | 676.61 | 0.002 | 7.25 | 0.0456 |
| 112 | 703.54 | 0.006 | 9.21 | 0.0764 |
| 113 | 715.01 | 0.010 | 34.60 | 0.0654 |
| 114 | 718.59 | 0.021 | 169.76 | 0.2701 |
| 115 | 726.41 | 0.019 | 135.88 | 0.2049 |
| 116 | 789.41 | 0.002 | 514.36 | 0.0146 |
| 117 | 808.11 | 0.001 | 62.81 | 0.0116 |
| 118 | 823.42 | 0.002 | 43.22 | 0.0679 |
| 119 | 830.73 | 0.001 | 20.25 | 0.0899 |
| 120 | 841.04 | 0.002 | 10.40 | 0.0124 |
| 121 | 843.98 | 0.001 | 34.60 | 0.0775 |
| 122 | 845.61 | 0.001 | 99.00 | 0.0847 |
| 123 | 851.20 | 0.002 | 106.04 | 0.2365 |
| 124 | 856.37 | 0.001 | 53.05 | 0.0818 |
| 125 | 891.65 | 0.001 | 2.67 | 0.0135 |
| 126 | 910.48 | 0.000 | 38.95 | 0.0074 |
| 127 | 925.61 | 0.002 | 18.83 | 0.0877 |
| 128 | 929.00 | 0.002 | 34.85 | 0.0863 |
| 129 | 946.44 | 0.002 | 22.95 | 0.0603 |
| 130 | 948.48 | 0.002 | 44.47 | 0.0875 |
| 131 | 957.48 | 0.002 | 44.90 | 0.0717 |
| 132 | 965.21 | 0.003 | 33.26 | 0.0441 |
| 133 | 978.33 | 0.002 | 38.16 | 0.1191 |
| 134 | 992.95 | 0.005 | 8.23 | 0.0045 |
| 135 | 998.23 | 0.002 | 28.26 | 0.0549 |

### E. Environment

Each central $HoW_{10}$ is surrounded by a layer of 18 $HoW_{10}$ units. The distances between the central Ho to the neighbouring Ho atoms are listed in the Table S4. We chose to surround the central $HoW_{10}$ unit with 10 neighbours, because there is an abrupt increase in distance (of 3.235 Å) from the $10^{th}$ neighbour to the $11^{th}$; see Fig. S9.

For the calculation of electrical dipole moment, we replaced the environment with point-charges, as shown in Fig. S10. The electric dipole was calculated in the presence of the environment not only at the optimized geometry but also at a series of distorted geometries from the equilibrium optimized geometry, following the displacement vectors of each vibrational mode. In each calculation we extracted the electric dipole of $HoW_{10}$. Fig. S11 and S12 show the results for the optimized geometry. The analogous calculations are represented in Fig. S15 and S16 for the crystal geometry.

For each distorted structure, the combination of the calculated force constant and the change in electric dipole compared with the undistorted structure allows us, employing the equations indicated above, to estimate the external electric field that would be needed to achieve said distortion. Thus, we can associate an $E$-field to every degree of

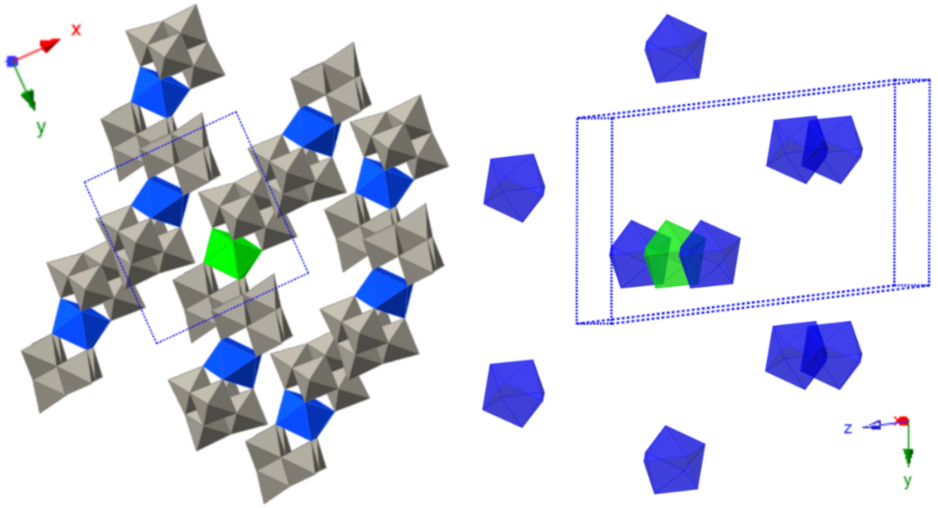


FIG. S9. Left: Packing diagram of anionic $HoW_{10}$ component in the crystal structure viewed along the $c$-axis using polyhedral representation. Blue (surrounding 10 Ho atoms) and green (one central Ho atom) square antiprism, $HoO_8$ units; Grey octahedra, $WO_6$. For clarity, sodium ions and water molecules are not shown. Right: Packing diagram of Ho atoms in the crystal structure using polyhedral representation. Blue (surrounding 10 Ho atoms) and green (one central Ho atom) square antiprism $HoO_8$ units.

distortion of each normal mode of the optimized structure shown in Fig. S13 and S14. The analogous calculations for the crystal geometry are represented in Fig. S17 and S18.

TABLE S4. The Ho-Ho distances for a given $HoW_{10}$ molecule and its 18 nearest neighbours

| $n^{th}$ neighbour | Ho-Ho distance (Å) | $n^{th}$ neighbour | Ho-Ho distance (Å) |
|---|---|---|---|
| 1 | 11.212 | 10 | 13.443 |
| 2 | 12.478 | 11 | 16.678 |
| 3 | 12.734 | 12 | 17.25 |
| 4 | 12.734 | 13 | 18.069 |
| 5 | 12.93 | 14 | 18.069 |
| 6 | 13.074 | 15 | 18.431 |
| 7 | 13.074 | 16 | 18.431 |
| 8 | 13.239 | 17 | 18.434 |
| 9 | 13.422 | 18 | 18.6 |

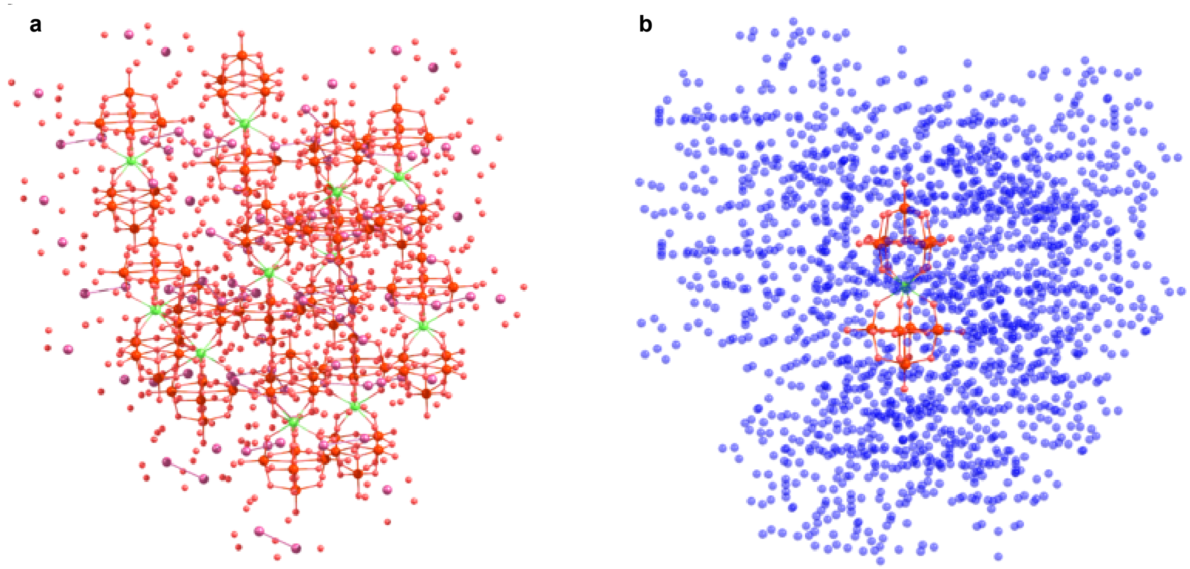


FIG. S10. (a) The fragment of $11\times(Na_9[Ho(W_5O_{18})_2]\cdot 35H_2O)$ on their crystallographic coordinates as employed to provide an environment to the central polyoxometalate; for clarity, hydrogen atoms are not shown. (b) Simplified system to model the electrostatic potential offered by environment, where all external entities $10\times Na_9[Ho(W_5O_{18})_2]\cdot 35H_2O$ as well as the nine $Na^+$ countercations and thirty-five crystallization water molecules of the central polyoxometalate are replaced by point charges (blue).

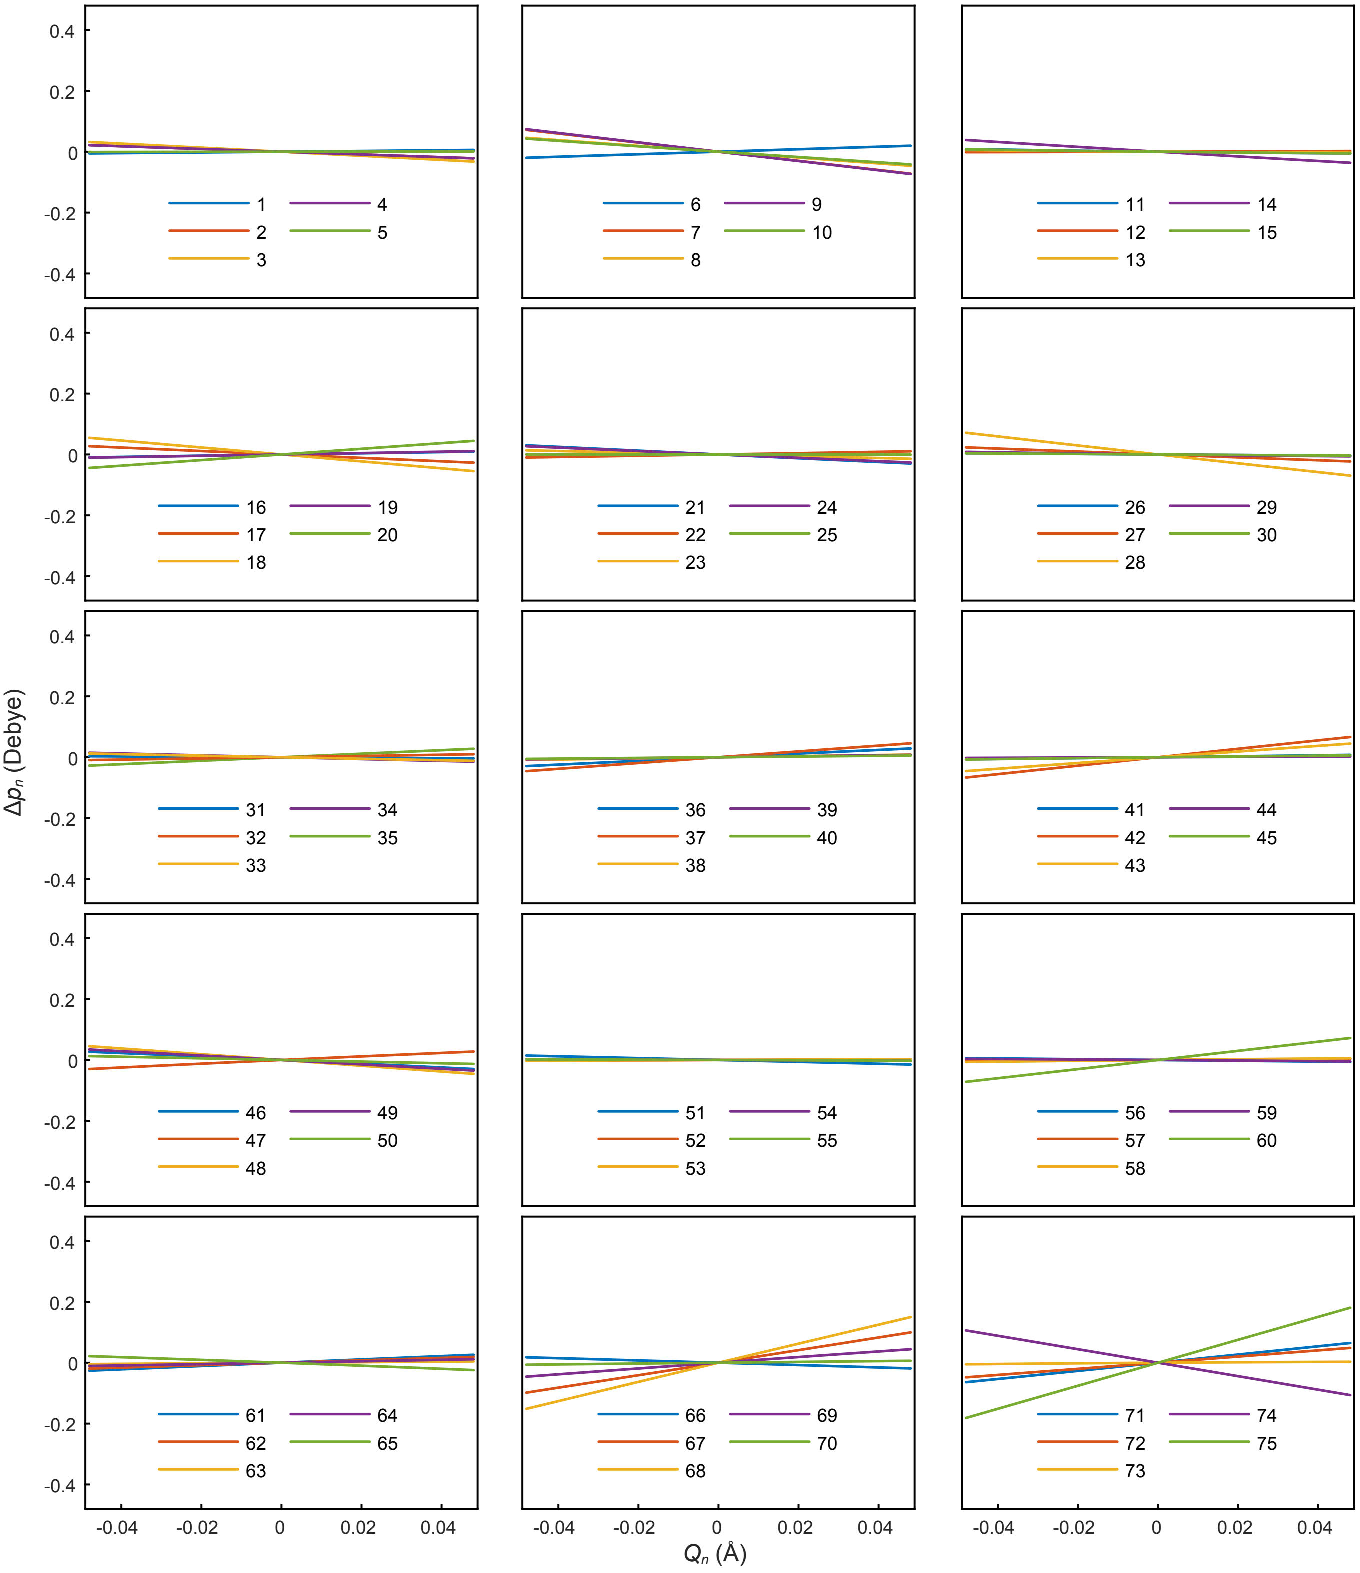


FIG. S11. Change in dipole moment $\Delta p_n$ for normal modes 1-75 for the optimized structure.

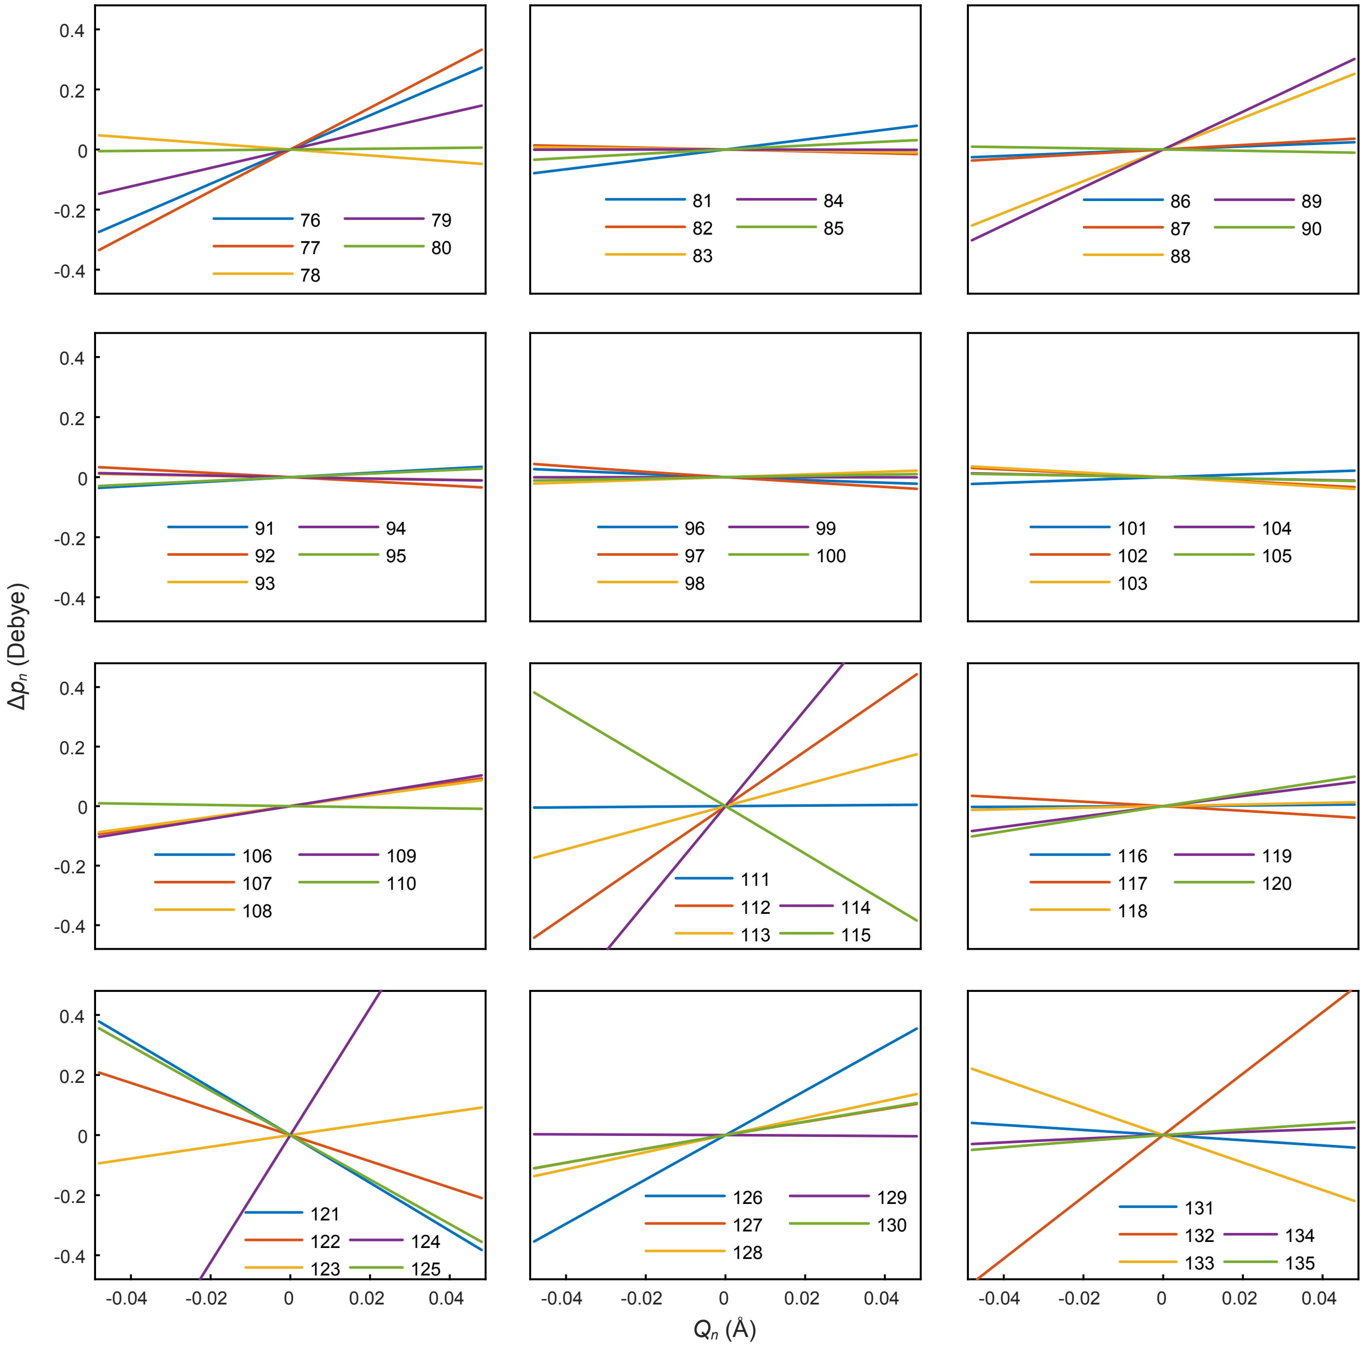


FIG. S12. Change in dipole moment $\Delta p_n$ for normal modes 76-135 for the optimized structure.

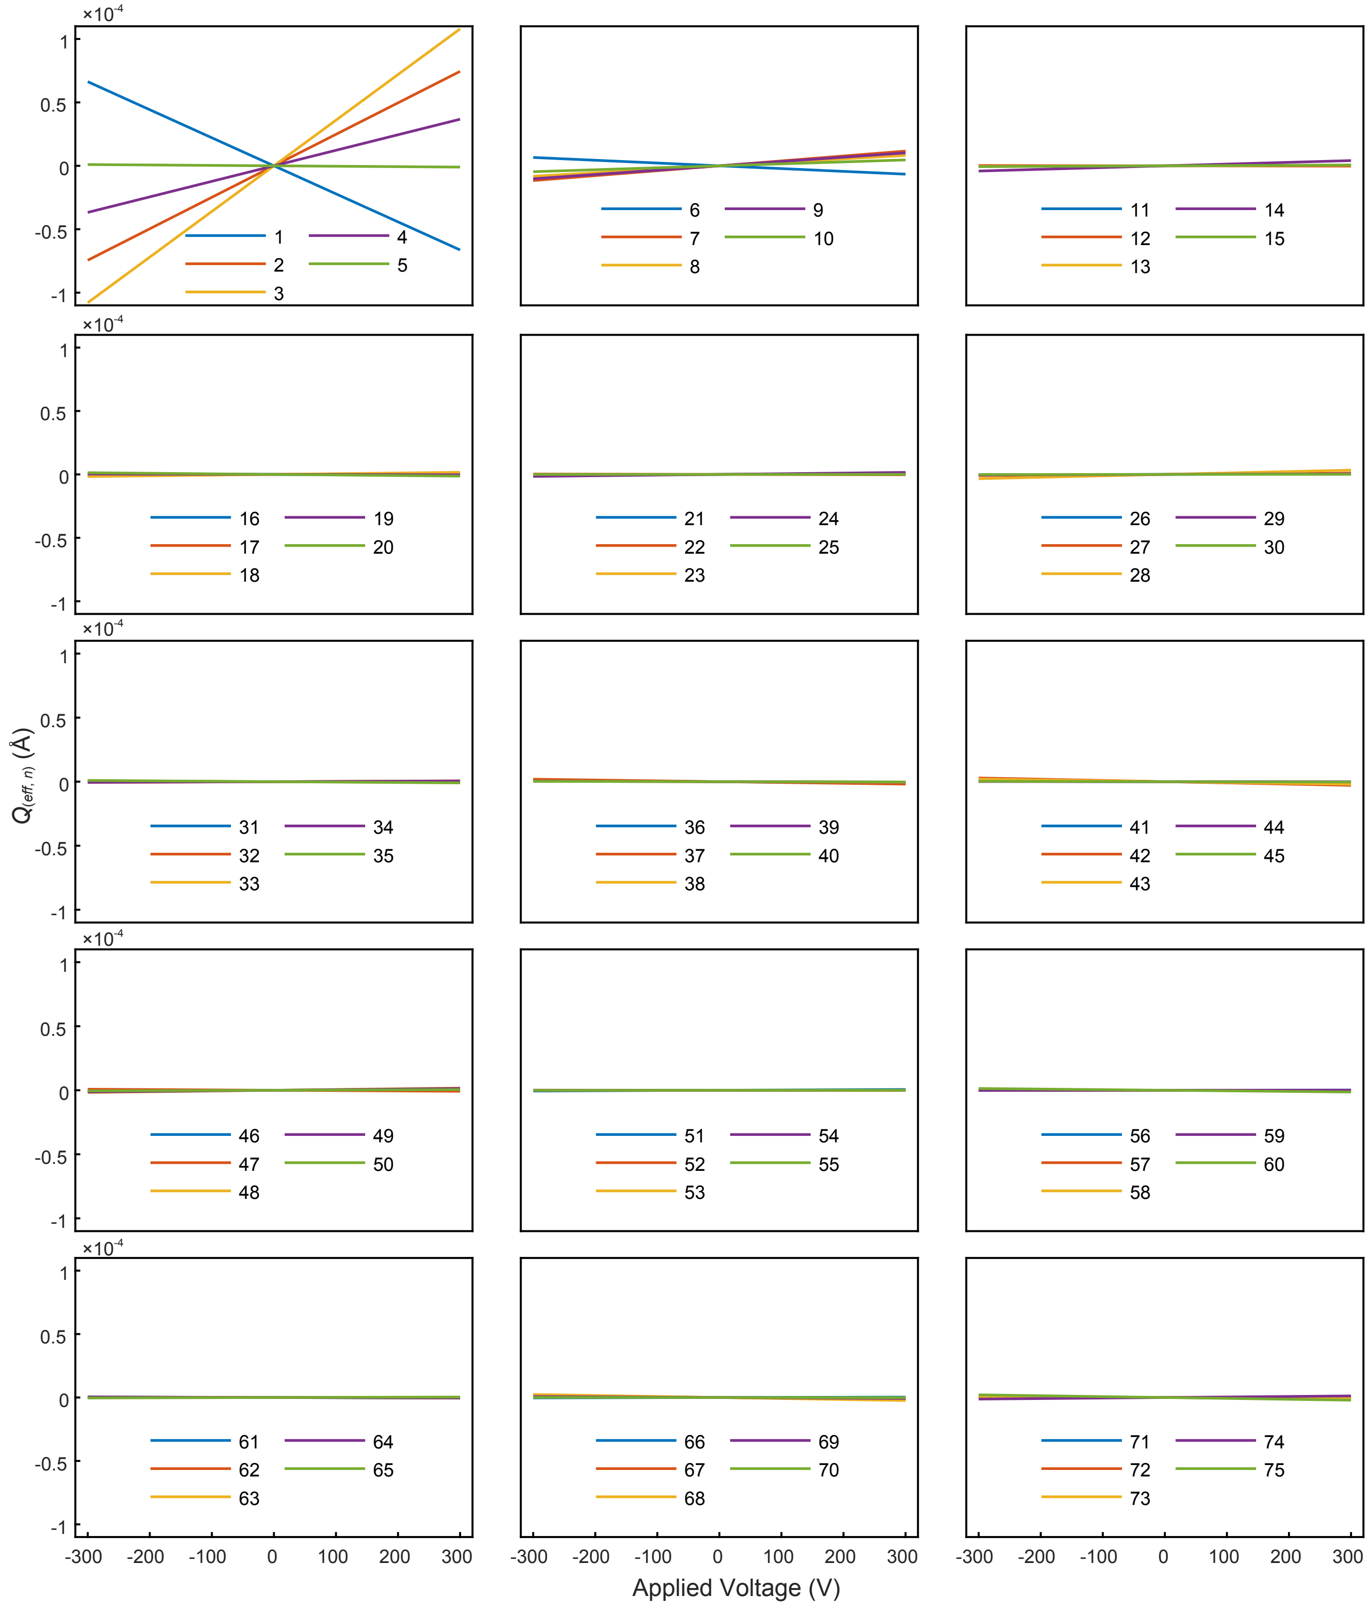


FIG. S13. Effective distortion attained by normal modes 1-75 of the optimized structure at applied voltages.

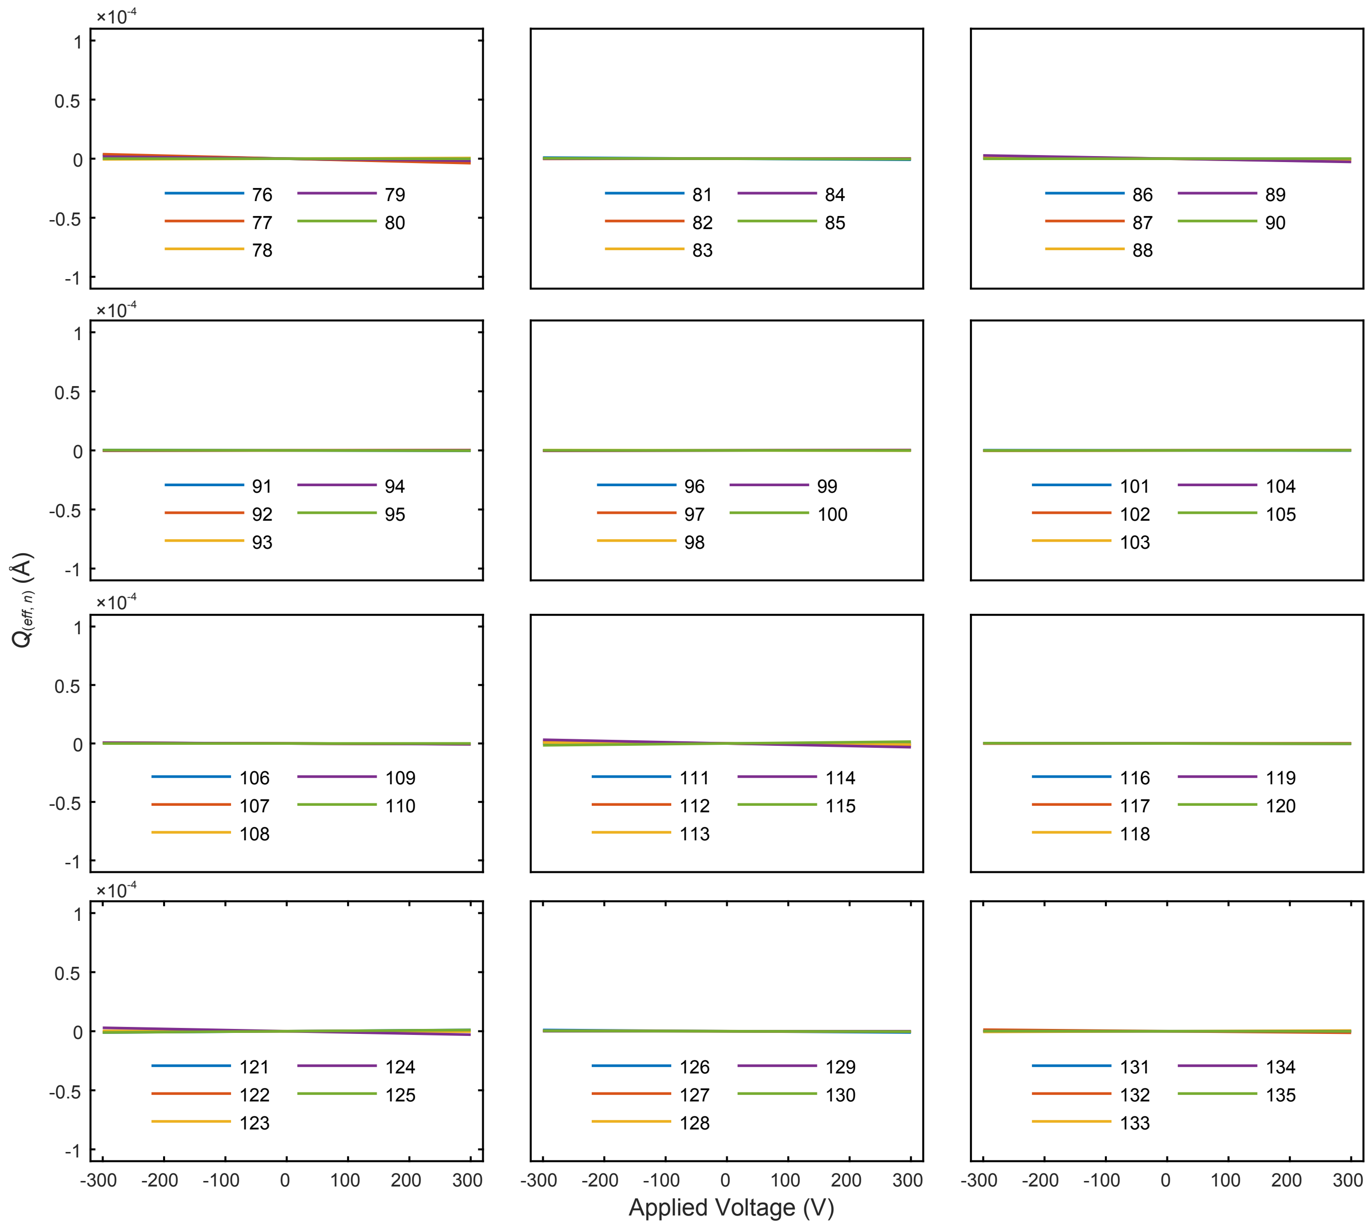


FIG. S14. Effective distortion attained by normal modes 76-135 of the optimized structure at applied voltages.

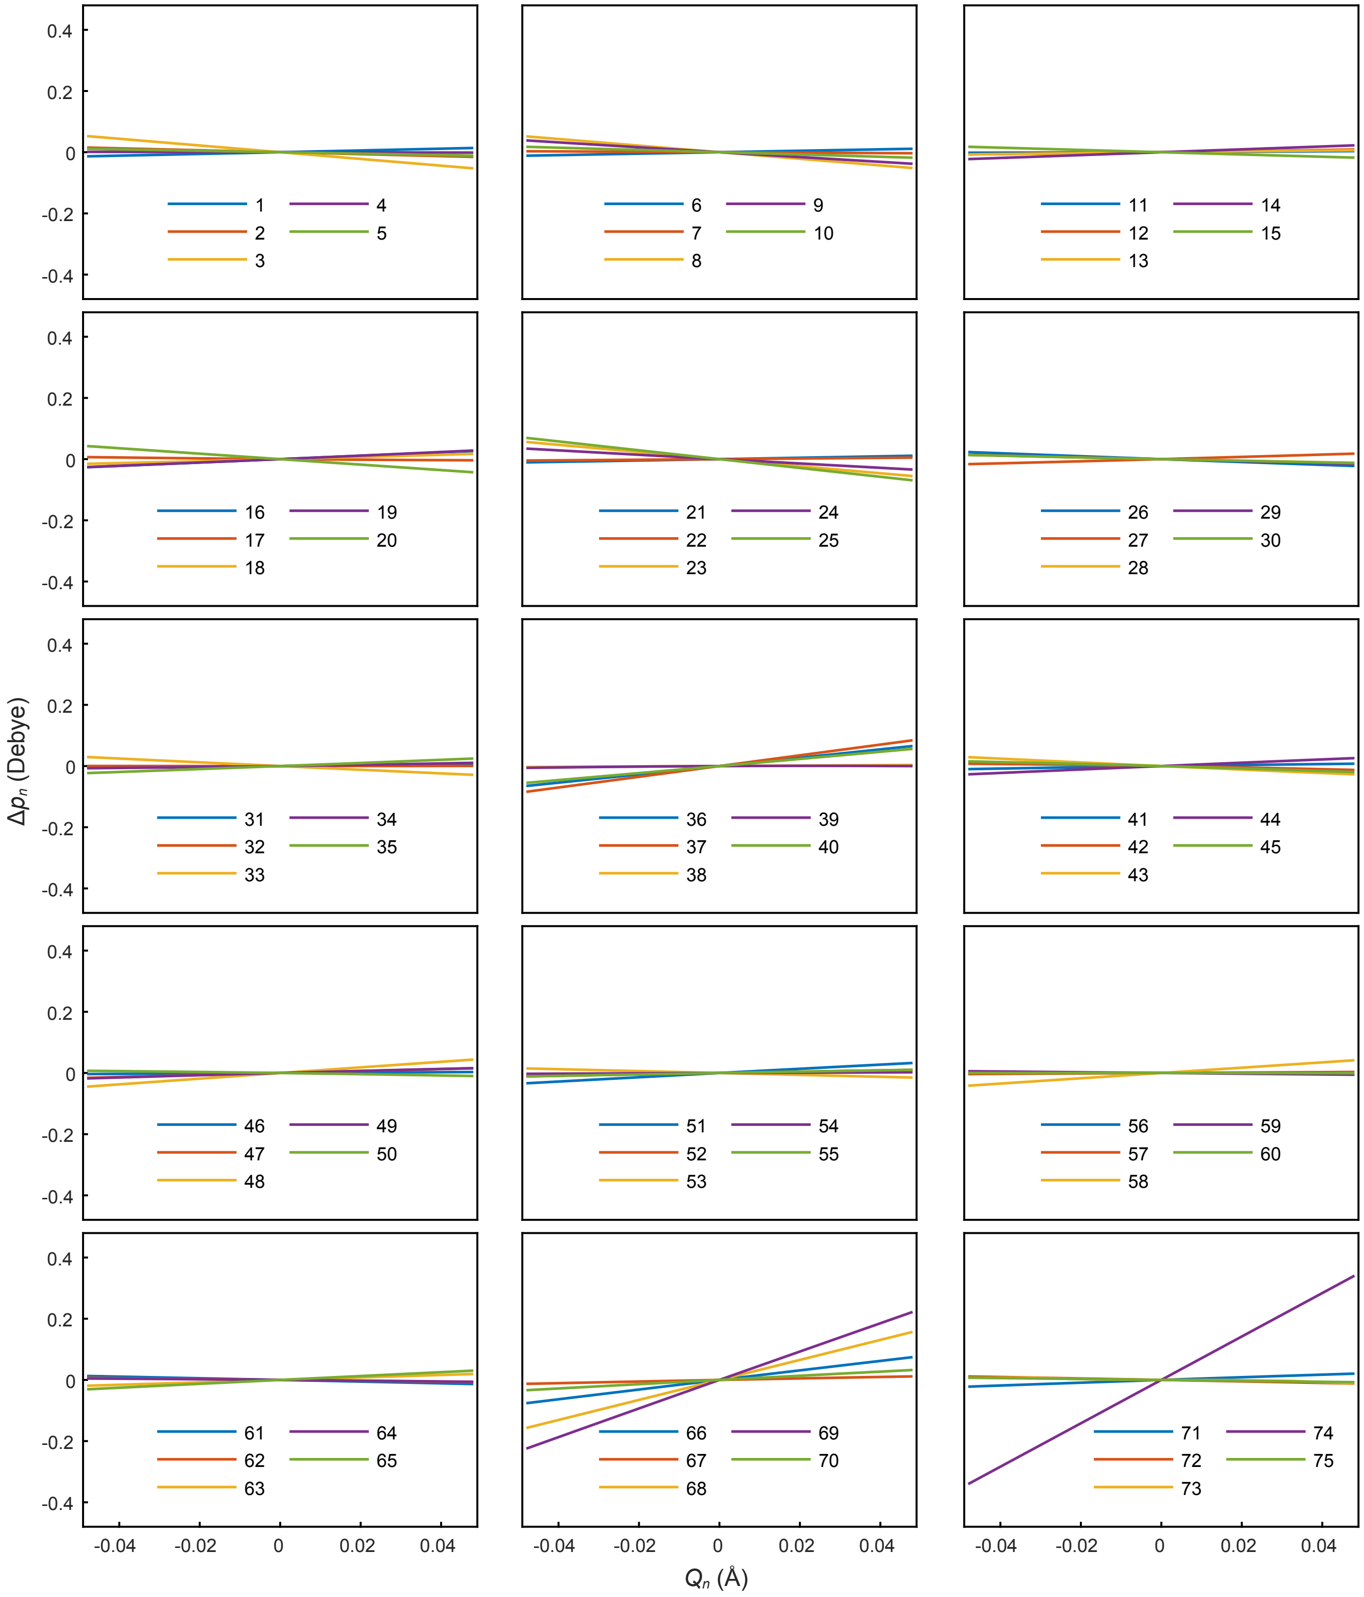


FIG. S15. Change in dipole moment $\Delta p_n$ for normal modes 1-75 for the crystal structure.

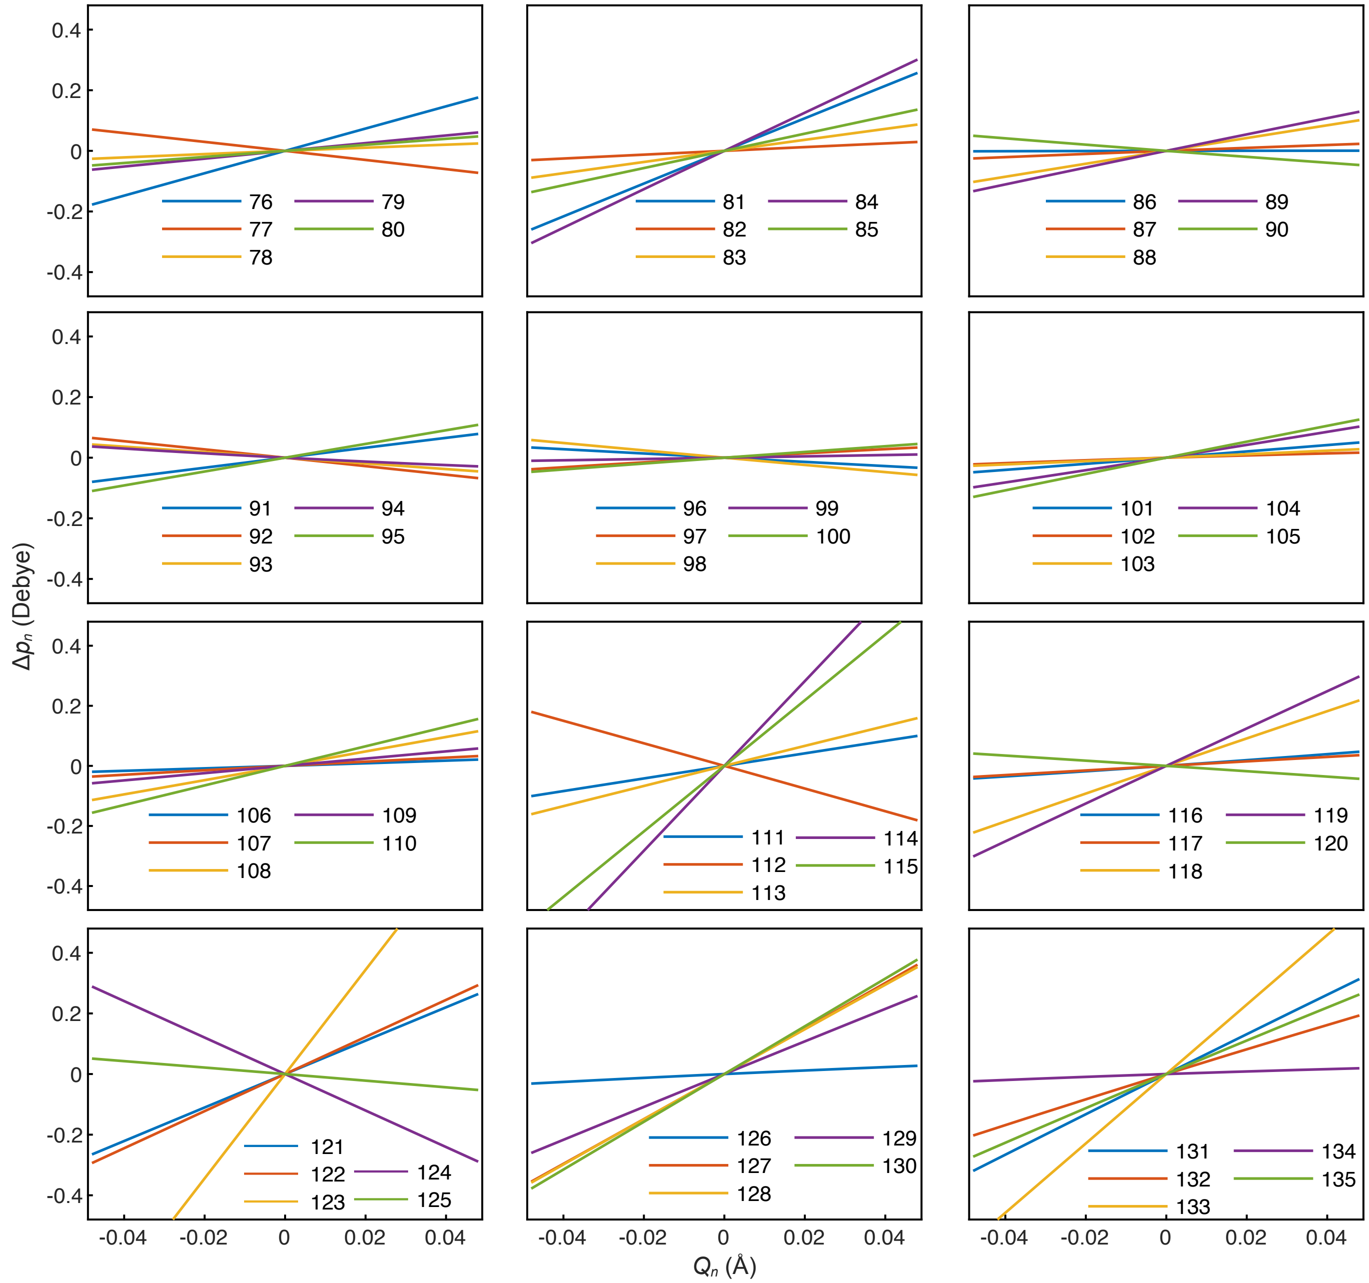


FIG. S16. Change in dipole moment $\Delta p_n$ for normal modes 76-135 for the crystal structure.

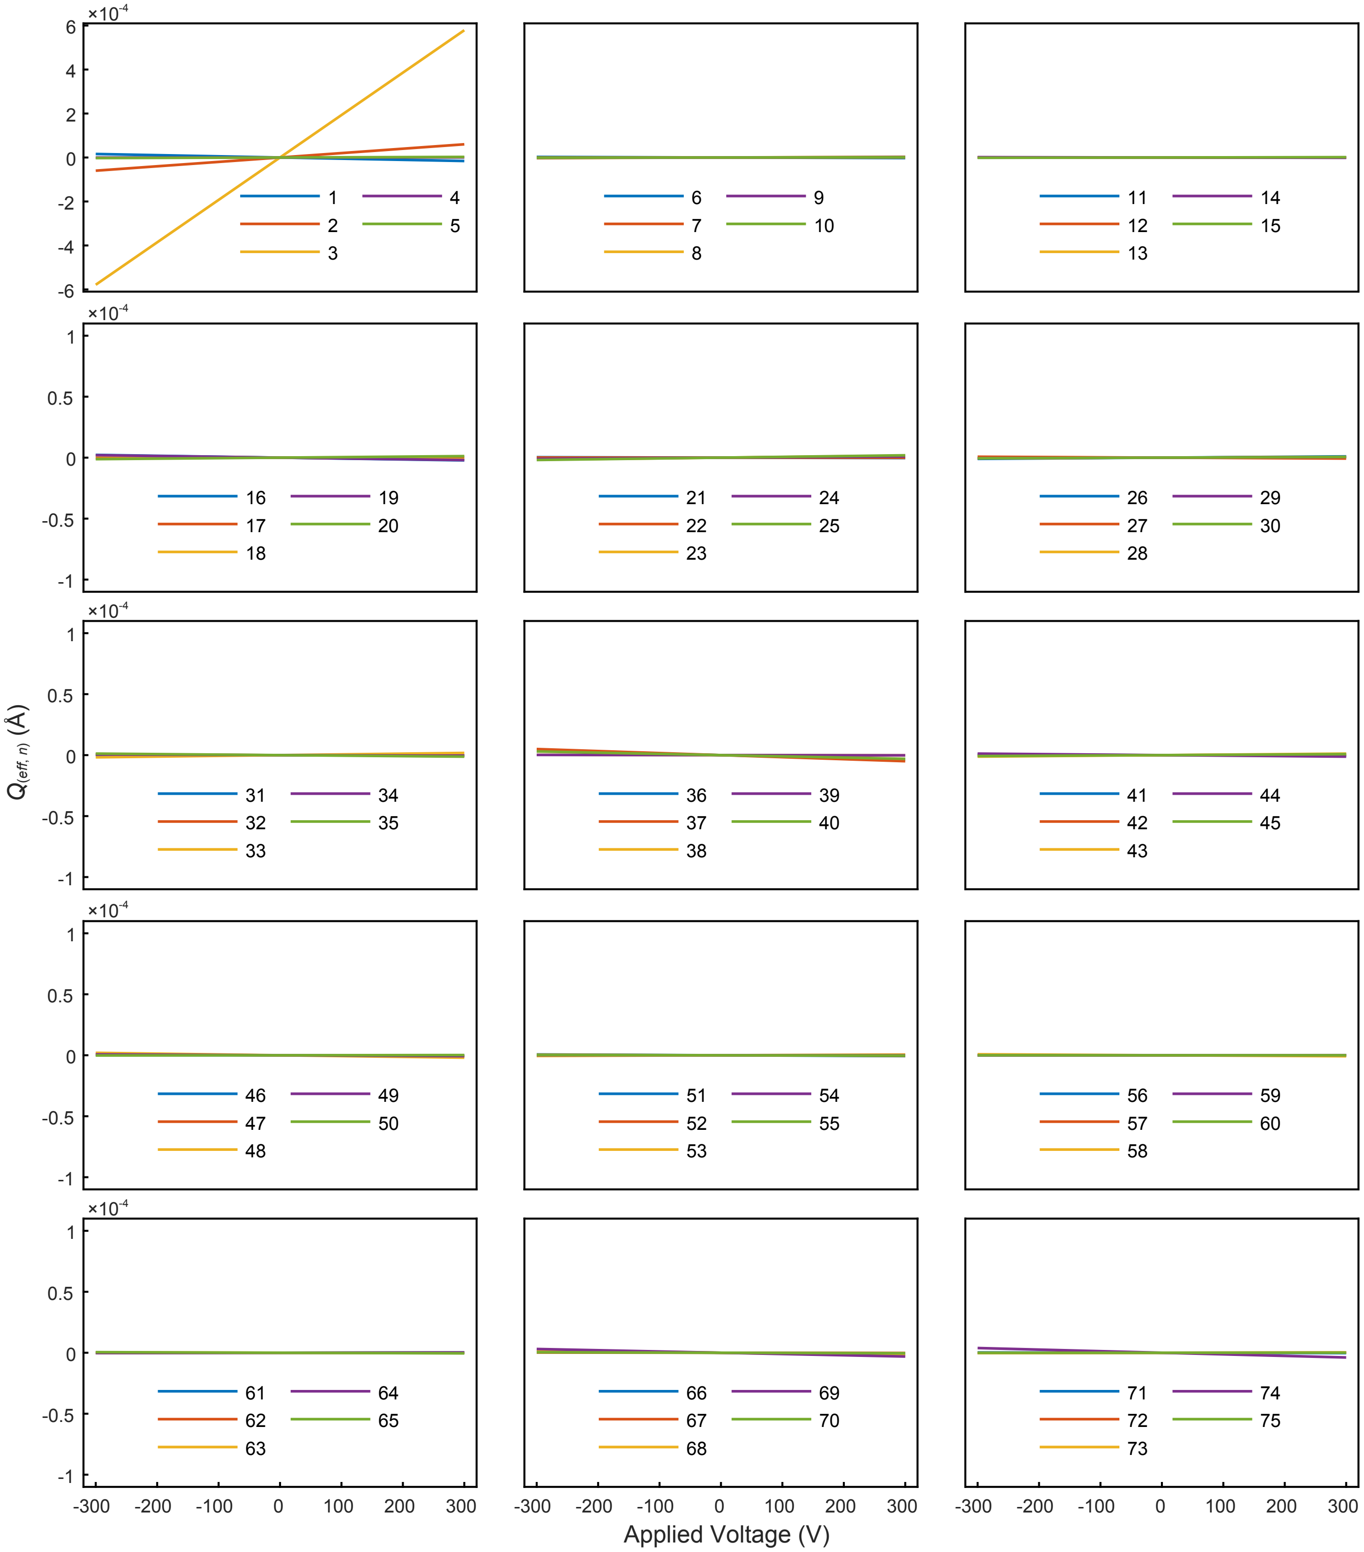


FIG. S17. Effective distortion attained by normal modes 1-75 of the crystal structure at applied voltages.

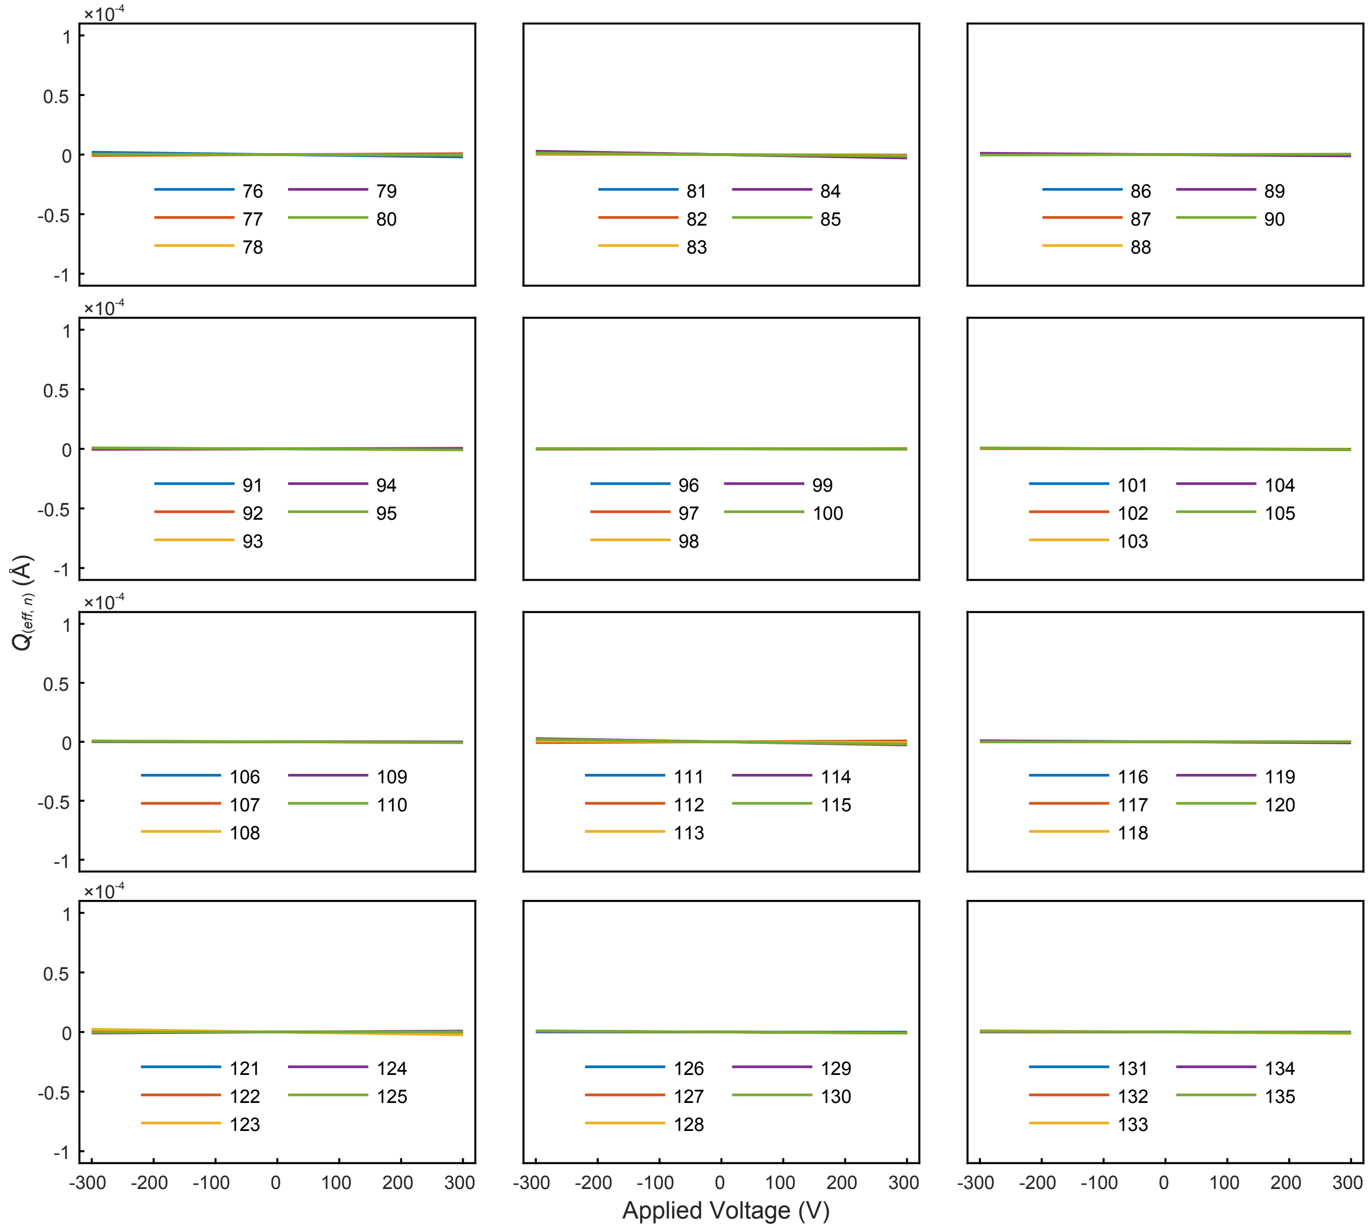


FIG. S18. Effective distortion attained by normal modes 76-135 of the crystal structure at applied voltages.

### F. Step 3: Determination of Spin energy Spectrum

*Ab-initio* calculations were performed to determine the spin energy level scheme, both in terms of the energies and in the composition of the ground state wave function in terms of $M_J$. Obtained results are provided in Table S5, both at crystallographic geometry and at the relaxed geometry.

TABLE S5. Energy level scheme (in $cm^{-1}$) and predominant $M_J$ microstate of the ground multiplet of the $HoW_{10}$ complex calculated (CASSCF) on the crystalline coordinates (left) and on the optimized coordinates (right).

| $E^{(a)}{}_{CASSCF}(cm^{-1})$ | $M_J$ | $E^{(b)}{}_{CASSCF}(cm^{-1})$ | $M_J$ |
|---|---|---|---|
| 0.00 | 47.5% $\|\pm4\rangle$ | 0.000 | 11.2% $\|\pm5\rangle$ + 12.2% $\|\pm6\rangle$ |
| 0.36 | 47.5% $\|\pm4\rangle$ | 0.022 | 13% $\|\pm5\rangle$ + 11.6% $\|\pm6\rangle$ |
| 26.24 | 47.2% $\|\pm3\rangle$ | 10.901 | 19.2% $\|\pm3\rangle$ |
| 27.92 | 47.2% $\|\pm3\rangle$ | 10.951 | 20.7% $\|\pm6\rangle$ + 14.7% $\|0\rangle$ |
| 50.08 | 48.7% $\|\pm5\rangle$ | 17.490 | 23.2% $\|\pm5\rangle$ + 10.2% $\|\pm1\rangle$ |
| 50.31 | 48.7% $\|\pm5\rangle$ | 17.512 | 24.6% $\|\pm4\rangle$ + 17.3% $\|0\rangle$ |
| 86.70 | 48.2% $\|\pm2\rangle$ | 53.364 | 26.5% $\|\pm7\rangle$ + 10.7% $\|\pm1\rangle$ |
| 96.34 | 48.2% $\|\pm2\rangle$ | 53.481 | 11.9% $\|\pm8\rangle$ + 10.9% $\|6\rangle$ |
| 155.59 | 48.9% $\|\pm1\rangle$ | 63.700 | 25.7% $\|\pm3\rangle$ + 10.2% $\|\pm1\rangle$ |
| 156.90 | 48.9% $\|\pm1\rangle$ | 63.707 | 16.4% $\|\pm4\rangle$ + 24.2% $\|\pm2\rangle$ |
| 178.90 | 46.6% $\|\pm6\rangle$ | 85.863 | 24.2% $\|\pm2\rangle$ + 33.5% $\|0\rangle$ |
| 179.05 | 46.6% $\|\pm6\rangle$ | 85.867 | 12.7% $\|\pm3\rangle$ + 31.8% $\|\pm1\rangle$ |
| 181.88 | 94.3% $\|0\rangle$ | 92.193 | 22.9% $\|\pm8\rangle$ + 18.6% $\|0\rangle$ |
| 279.97 | 49.3% $\|\pm8\rangle$ | 93.320 | 23.9% $\|\pm7\rangle$ + 16.8% $\|\pm5\rangle$ |
| 279.97 | 49.3% $\|\pm8\rangle$ | 124.856 | 11.1% $\|\pm3\rangle$ + 11.5% $\|\pm1\rangle$ |
| 315.99 | 49.1% $\|\pm7\rangle$ | 126.665 | 27.4% $\|\pm8\rangle$ |
| 315.99 | 49.1% $\|\pm7\rangle$ | 138.346 | 20.3% $\|\pm8\rangle$ + 10.3% $\|\pm6\rangle$ |

### G. Step 4: Effects of the $E$-field on the tunneling splitting

Finally, we were able to determine the change in the clock-transition frequency ($\delta f$) by evaluating the evolution of the tunnel splitting at CASSCF level. The calculations were performed for both crystal and optimized structures see Fig. S19. A clear linear evolution of $\delta f$ is observed for both structures, both compatible with experimental results. For both structures, the strongest SEC is found when the $E$-field is applied parallel to the molecular electric dipole, as shown in Fig. S19a and b. The DFT calculations show that the molecular electric dipole is tilted 42° and 54° away from the pseudo tetragonal axis for the optimised and crystal structures, respectively.

This difference can be understood by considering the following symmetry considerations. Since a linear effect of the voltage in the tunneling splitting requires a pre-existing inversion symmetry breaking, in an ideal $D_{4d}$ system the effect would be zero in the first order and only present as a second-order contribution. The relaxed geometry is closer to the ideal $D_{4d}$ symmetry compared with the crystal structure (which is influenced by nearby $Na^+$ counterions and crystallization $H_2O$ molecules) and thus the effect of an external distortion on its tunnel splitting is underestimated.

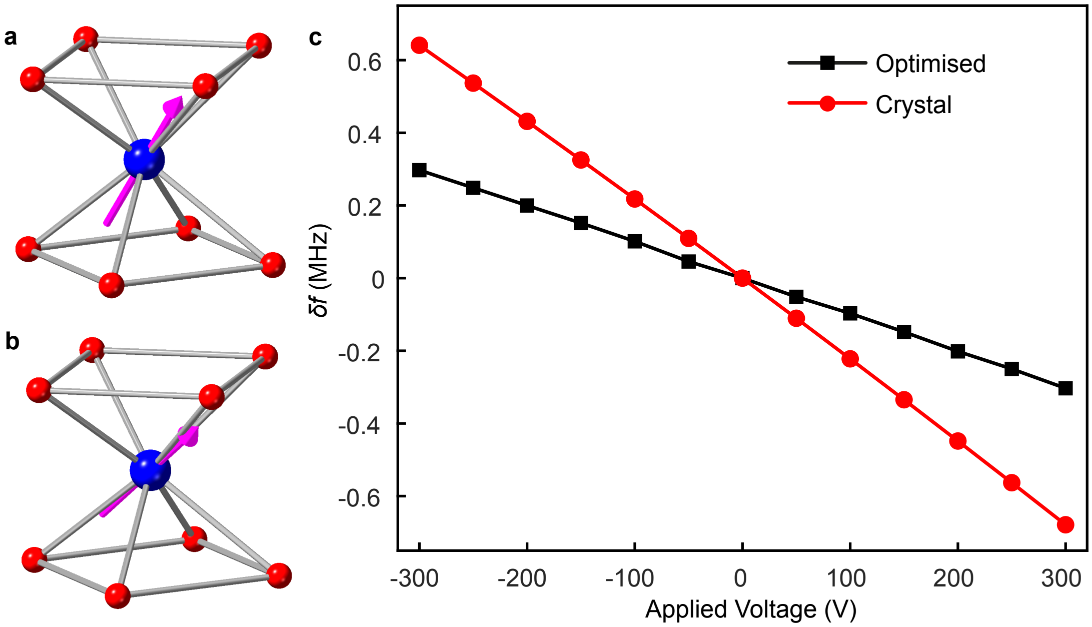


FIG. S19. (a) and (b) The local environment of the Ho, showing the calculated electric dipole direction (magenta arrow) for the optimised and crystal structures, respectively. (c) Change in clock-transition $\delta f$ as a function of the applied voltage. The black and red symbols correspond to the results calculated using the optimised and crystal structures, respectively.

Additionally we computed the deviation of the easy axis orientation as a function of the applied voltage at CASSCF-SO level (Table S6). At 300 V we obtain deviations of $\delta = 1.27°$ and 0.14° for the optimized and crystallographic structures, respectively. This results in a deviation in the effective field of $\cos(\delta) \cdot B_{\mathrm{CT}}$. Since the frequency response is quadratic in the vicinity of the CTs, this translates into changes $k((1-\cos(\delta)) \cdot B_{\mathrm{CT}})^2$, where $k = 36$ cm$^{-1}$T$^{-2}$ [S8] and $B_{\mathrm{CT}}$ is $B_{\min} = 0.0236$, 0.0709, 0.1181 and 0.1654 T. Thus, this effect is in the ranges $1.26 \times 10^{-9}$ to $6.23 \times 10^{-8}$ cm$^{-1}$ (optimized) and $2.10 \times 10^{-13}$ to $1.03 \times 10^{-11}$ cm$^{-1}$ (crystallographic), i.e. below 0.002 MHz.

TABLE S6. Calculated deviation of the easy axis orientation as a function of the applied voltage.

| Voltage (V) | $\delta_{\mathrm{OPT}}$ (degrees) | $\delta_{\mathrm{CRYS}}$ (degrees) |
|---|---|---|
| -300 | -1.276 | -0.137 |
| -250 | -1.064 | -0.115 |
| -200 | -0.852 | -0.092 |
| -150 | -0.639 | -0.069 |
| -100 | -0.427 | -0.046 |
| -50 | -0.213 | -0.023 |
| 0 | 0.000 | 0.000 |
| 50 | 0.213 | 0.023 |
| 100 | 0.426 | 0.047 |
| 150 | 0.641 | 0.071 |
| 200 | 0.855 | 0.096 |
| 250 | 1.070 | 0.120 |
| 300 | 1.285 | 0.145 |

### H. Step 5: Calculation of the angular dependency

As a first theoretical estimate of the angular dependence of the transition frequency at the clock transition, we started from Eqn. S15, where $\rho$ is the angle between applied electrical field and the dipole moment.

$$U_n = -\Delta p E \cos\rho \tag{S15}$$

Now, the effective distortion can be obtained by the changing the angle $\rho$ between the applied voltage and the dipole moment.

$$\vec{Q}_{\mathrm{eff}}(V(\rho)) = \sum_n Q_{(\mathrm{eff},n)}(V(\rho)) = Q_{(\mathrm{eff},1)}(V(\rho)) + Q_{(\mathrm{eff},2)}(V(\rho)) + .... + Q_{(\mathrm{eff},3N-6)}(V(\rho)) \tag{S16}$$

We started from the effective distortion obtained at -300V that is $\vec{Q}_{\mathrm{eff}}(-300V(0^\circ))$, and determined further angular dependent distortion at $\vec{Q}_{\mathrm{eff}}(-300V(30^\circ))$, $\vec{Q}_{\mathrm{eff}}(-300V(60^\circ))$, $\vec{Q}_{\mathrm{eff}}(-300V(90^\circ))$, $\vec{Q}_{\mathrm{eff}}(-300V(120^\circ))$, $\vec{Q}_{\mathrm{eff}}(-300V(150^\circ))$ and $\vec{Q}_{\mathrm{eff}}(-300V(180^\circ))$. At each distortion we performed CASSCF-SO calculations to determine the change in clock-transition frequency, obtained results are shown in Fig. S20.

As a proof of concept, if we start from -300V, the obtained electrically induced transition should reach to the value

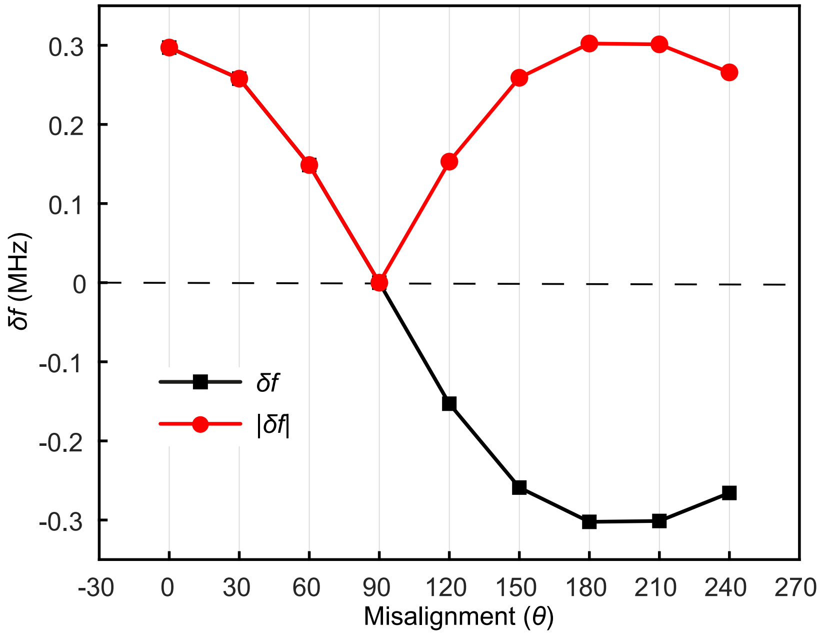


FIG. S20. Change in clock-transition $\delta f$ (MHz) for angular dependent distortion $\vec{Q}_{\text{eff}}(V(\rho))$ at 300V.

at +300V in linear effect obtained in Fig. S20.

---


[S1] Casanova, D. *et al.* Minimal distortion pathways in polyhedral rearrangements. *Journal of the American Chemical Society* **126**, 1755–1763 (2004).

[S2] Casanova, D., Llunell, M., Alemany, P. & Alvarez, S. The rich stereochemistry of eight-vertex polyhedra: A continuous shape measures study. *Chemistry – A European Journal* **11**, 1479–1494 (2005).

[S3] Troiani, F. Manipulation of spin cluster qubits by electric field induced modulation of exchange coupling, $g$-factor, and axial anisotropy. *Physical Review B* **100**, 155424 (2019).

[S4] Forrer, J., García-Rubio, I., Schuhmam, R., Tschaggelar, R. & Harmer, J. Cryogenic Q-band (35GHz) probehead featuring large excitation microwave fields for pulse and continuous wave electron paramagnetic resonance spectroscopy: Performance and applications. *Journal of Magnetic Resonance* **190**, 280–291 (2008).

[S5] Fdez. Galvan, I. *et al.* Openmolcas: From source code to insight. *Journal of chemical theory and computation* **15**, 5925–5964 (2019).

[S6] Ungur, L. & Chibotaru, L. F. Ab initio crystal field for lanthanides. *Chemistry–A European Journal* **23**, 3708–3718 (2017).

[S7] Frisch, M. J. *et al.* Gaussian 16 Revision A.03 (2016).

[S8] Giménez-Santamarina, S., Cardona-Serra, S., Clemente-Juan, J. M., Gaita-Ariño, A. & Coronado, E. Exploiting clock transitions for the chemical design of resilient molecular spin qubits. *Chemical Science* **11**, 10718–10728 (2020).
